# Supplementary material for: An Optimization Case Study for solving a Transport Robot Scheduling Problem on Quantum-Hybrid and Quantum-Inspired Hardware
Source: arXiv:2309.09736 source file (2023-10-24)
Supplement: Supplementary file 1 [file Supplementary-Material-Instance-Lists.pdf]

**Supplementary Table S5.** A list with all parameters of the minor instance library. The following abbrevations are used: conf-key: The configuration $(N, K, p_3)(nr)$ where $nr \in \{0, \ldots, 9\}$ is the number of the randomly generated instance; process times: the process times of the samples (columns) on sample shaker (row 1), sample mixer (row 2) and photo booth (row 3); gaps: the gaps between subsequent photos of the samples (columns), gap 1 between photo 1 and photo 2 is in row 1 and so on; number of variables (NV); runtime (T); objective value (OV); Time-indexed model (TI); Gurobi with the time-indexed model (TI-GU) Sequence model (S); Gurobi with the sequence model (SE-GU); QUBO model (Q);D-Wave's hybrid *Leap* framework (LBQM) with the QUBO model (QU-LBQM); Fujitsu's digital annealer (FDA) with the QUBO model (QU-FDA); the relative runtime of SE-GU w.r.t. QU-LBQM (SE-GU@QU-LBQM); the relative runtime of SE-GU w.r.t. QU-FDA (SE-GU@QU-FDA); the relative runtime of TI-GU w.r.t. QU-LBQM (TI-GU@QU-LBQM); the relative runtime of TI-GU w.r.t. QU-FDA (TI-GU@QU-FDA); feasibility (F) (number of penalties violated in LBQM solution, 0 iff feasible).

| conf-key | process times | gaps | NV-TI | T-TI-GU | OV-TI-GU | TI-GU@QU-LBQM | TI-GU@QU-FDA | NV-S | T-SE-GU | OV-SE-GU | SE-GU@QU-LBQM | SE-GU@QU-FDA | NV-Q | T-QU-FDA | OV-QU-FDA | T-QU-LBQM | OV-QU-LBQM | F-QU-LBQM |
|---|---|---|---|---|---|---|---|---|---|---|---|---|---|---|---|---|---|---|
| (4, 4, 1)(0) | 4 7 4 5<br>2 2 4 4<br>1 1 1 1 | 4 4 4 4<br>11 11 11 9<br>23 23 18 19 | 6564 | 184.72 | 345 | 20 | 25 | 1080 | 0.37 | 345 | 0 | 0 | 2166 | 5.97 | 444 | 32 | 471 | 0 |
| (4, 4, 1)(1) | 6 8 8 5<br>4 2 3 3<br>1 1 1 1 | 4 5 4 4<br>11 8 8 10<br>19 22 19 19 | 6532 | 52.78 | 334 | 19 | 19 | 1080 | 0.67 | 334 | 0 | 0 | 2149 | 6.07 | 429 | 32 | 495 | 0 |
| (4, 4, 1)(2) | 4 5 6 6<br>3 4 1 2<br>1 1 1 1 | 4 4 4 5<br>11 11 9 8<br>23 23 17 20 | 6468 | 65.39 | 333 | 17 | 21 | 1080 | 0.50 | 333 | 0 | 0 | 2137 | 5.09 | 414 | 32 | 520 | 0 |
| (4, 4, 1)(3) | 4 7 5 4<br>4 2 2 4<br>1 1 1 1 | 5 5 4 4<br>10 9 8 10<br>17 23 20 19 | 6340 | 41.62 | 302 | 17 | 18 | 1080 | 0.51 | 302 | 0 | 0 | 2096 | 4.98 | 407 | 31 | 477 | 0 |
| (4, 4, 1)(4) | 4 6 6 8<br>4 3 1 4<br>1 1 1 1 | 4 5 5 5<br>11 10 10 8<br>23 23 17 16 | 6564 | 128.13 | 316 | 16 | 16 | 1080 | 0.58 | 316 | 0 | 0 | 2162 | 6.07 | 440 | 32 | 514 | 0 |
| (4, 4, 1)(5) | 5 6 5 8<br>1 2 4 1<br>1 1 1 1 | 4 4 5 4<br>11 8 8 9<br>22 21 22 23 | 6564 | 131.44 | 334 | 19 | 19 | 1080 | 0.81 | 334 | 0 | 0 | 2166 | 5.98 | 425 | 32 | 458 | 0 |
| (4, 4, 1)(7) | 7 8 8 4<br>1 3 3 3<br>1 1 1 1 | 5 5 4 4<br>9 11 10 10<br>17 20 20 16 | 6404 | 57.18 | 319 | 18 | 20 | 1080 | 0.65 | 319 | 0 | 0 | 2111 | 5.12 | 404 | 31 | 477 | 0 |
| (4, 4, 1)(8) | 6 7 7 5<br>1 2 2 2<br>1 1 1 1 | 5 5 4 5<br>9 11 9 11<br>23 20 21 21 | 6660 | 152.29 | 329 | 19 | 20 | 1080 | 0.60 | 329 | 0 | 0 | 2196 | 6.21 | 418 | 32 | 498 | 0 |
| (4, 4, 1)(9) | 7 8 5 7<br>3 4 1 4<br>1 1 1 1 | 4 5 4 5<br>9 11 9 10<br>19 16 20 19 | 6468 | 49.53 | 325 | 19 | 20 | 1080 | 0.41 | 325 | 0 | 0 | 2129 | 5.05 | 426 | 31 | 472 | 0 |
| (4, 4, 3)(0) | 5 7 7 8<br>2 2 2 1<br>3 3 3 3 | 5 4 4 5<br>10 8 9 8<br>18 17 19 23 | 6916 | 60.98 | 384 | 28 | 28 | 1080 | 0.62 | 384 | 0 | 0 | 2410 | 6.56 | 496 | 36 | 540 | 0 |
| (4, 4, 3)(1) | 6 8 4 6<br>2 2 4 1<br>3 3 3 3 | 4 4 5 5<br>9 9 11 10<br>16 20 23 20 | 7076 | 63.72 | 400 | 31 | 35 | 1080 | 0.33 | 400 | 0 | 0 | 2461 | 6.69 | 477 | 36 | 558 | 0 |
| (4, 4, 3)(2) | 4 4 7 8<br>2 3 1 4<br>3 3 3 3 | 4 4 4 4<br>10 11 11 8<br>19 23 21 19 | 7140 | 58.90 | 391 | 29 | 31 | 1080 | 0.52 | 391 | 0 | 0 | 2481 | 6.58 | 517 | 37 | 622 | 0 |
| (4, 4, 3)(3) | 7 6 8 4<br>4 2 4 2<br>3 3 3 3 | 5 5 4 4<br>11 8 11 8<br>22 19 21 17 | 7172 | 59.54 | 382 | 31 | 41 | 1080 | 0.73 | 382 | 0 | 0 | 2487 | 6.66 | 477 | 37 | 581 | 0 |
| (4, 4, 3)(4) | 5 6 7 7<br>1 3 4 3<br>3 3 3 3 | 5 5 5 5<br>10 8 11 9<br>16 18 22 22 | 7172 | 64.05 | 381 | 35 | 40 | 1080 | 0.56 | 381 | 0 | 0 | 2488 | 6.60 | 487 | 37 | 579 | 0 |
| (4, 4, 3)(5) | 7 7 4 4<br>4 2 3 4<br>3 3 3 3 | 4 5 5 4<br>8 8 10 8<br>18 20 20 18 | 6916 | 52.51 | 380 | 32 | 37 | 1080 | 0.93 | 380 | 0 | 0 | 2399 | 6.47 | 481 | 35 | 550 | 0 |
| (4, 4, 3)(6) | 8 4 7 6<br>3 3 1 1<br>3 3 3 3 | 4 5 4 5<br>9 9 9 10<br>19 20 20 17 | 6916 | 59.21 | 381 | 25 | 28 | 1080 | 0.78 | 381 | 0 | 0 | 2411 | 6.65 | 501 | 36 | 614 | 0 |
| (4, 4, 3)(7) | 4 5 5 5<br>2 4 3 1<br>3 3 3 3 | 4 4 4 5<br>9 11 11 8<br>16 16 21 20 | 6756 | 55.49 | 376 | 25 | 26 | 1080 | 0.74 | 376 | 0 | 0 | 2355 | 6.36 | 500 | 35 | 533 | 0 |
| (4, 4, 3)(8) | 5 6 4 5<br>3 1 3 3<br>3 3 3 3 | 5 4 4 4<br>10 9 11 9<br>17 17 20 16 | 6692 | 50.70 | 368 | 28 | 28 | 1080 | 0.83 | 368 | 0 | 0 | 2334 | 6.26 | 479 | 35 | 485 | 0 |
| (4, 4, 3)(9) | 8 4 7 6<br>4 2 4 2<br>3 3 3 3 | 5 4 4 5<br>8 9 9 8<br>16 18 18 19 | 6820 | 54.75 | 364 | 27 | 36 | 1080 | 0.35 | 364 | 0 | 0 | 2367 | 6.41 | 444 | 35 | 556 | 0 |
| (5, 3, 1)(3) | 8 5 7 7 8<br>1 3 1 4 3<br>1 1 1 1 1 | 5 4 4 5 5<br>8 9 10 10 9 | 6045 | 234.34 | 320 | 11 | 11 | 1330 | 0.76 | 320 | 0 | 0 | 2071 | 4.94 | 399 | 31 | 432 | 0 |
| (5, 3, 1)(4) | 8 5 8 7 5<br>4 1 2 2 2<br>1 1 1 1 1 | 4 5 4 5 4<br>11 11 9 9 10 | 6045 | 247.01 | 321 | 11 | 13 | 1330 | 0.66 | 321 | 0 | 0 | 2074 | 4.91 | 372 | 31 | 449 | 0 |
| (5, 3, 1)(5) | 7 5 4 5 5<br>4 4 4 4 4<br>1 1 1 1 1 | 4 5 5 4 5<br>11 10 9 11 11 | 6245 | 205.48 | 327 | 13 | 14 | 1330 | 0.70 | 327 | 0 | 0 | 2137 | 5.01 | 388 | 32 | 449 | 0 |
| (5, 3, 1)(7) | 8 6 7 6 7<br>2 3 4 3 3<br>1 1 1 1 1 | 4 4 4 4 4<br>10 11 9 11 11 | 6245 | 1464.35 | 379 | 12 | 14 | 1330 | 0.66 | 379 | 0 | 0 | 2134 | 4.98 | 408 | 32 | 452 | 0 |
| (5, 3, 1)(8) | 6 7 7 8 8<br>2 3 1 2 4<br>1 1 1 1 1 | 4 5 5 5 4<br>8 11 10 8 9 | 6085 | 354.10 | 322 | 11 | 11 | 1330 | 0.91 | 322 | 0 | 0 | 2083 | 5.04 | 400 | 31 | 421 | 0 |
| (5, 3, 3)(0) | 5 5 4 8 5<br>1 1 3 1 1<br>3 3 3 3 3 | 5 4 4 4 5<br>8 9 11 9 11 | 6765 | 245.03 | 420 | 16 | 20 | 1330 | 0.51 | 420 | 0 | 0 | 2338 | 6.17 | 454 | 35 | 504 | 0 |
| (5, 3, 3)(1) | 6 6 4 5 4<br>1 2 1 3 4<br>3 3 3 3 3 | 4 4 5 5 4<br>10 9 8 10 8 | 6725 | 194.32 | 412 | 16 | 28 | 1330 | 0.57 | 412 | 0 | 0 | 2323 | 6.23 | 450 | 34 | 491 | 0 |
| (5, 3, 3)(2) | 4 6 4 7 7<br>2 4 1 1 4<br>3 3 3 3 3 | 4 4 5 5 4<br>9 10 11 11 8 | 7045 | 234.95 | 423 | 16 | 21 | 1330 | 0.68 | 423 | 0 | 0 | 2423 | 6.37 | 476 | 36 | 489 | 0 |
| (5, 3, 3)(3) | 5 4 8 4 8<br>3 4 3 3 4<br>3 3 3 3 3 | 5 5 4 4 4<br>8 10 11 8 10 | 7205 | 151.77 | 418 | 17 | 18 | 1330 | 0.74 | 418 | 0 | 0 | 2469 | 6.50 | 493 | 37 | 526 | 0 |
| (5, 3, 3)(4) | 4 7 5 4 4<br>1 1 1 2 4<br>3 3 3 3 3 | 5 4 5 4 4<br>9 10 10 8 8 | 6605 | 202.11 | 413 | 15 | 17 | 1330 | 0.55 | 413 | 0 | 0 | 2287 | 6.03 | 455 | 34 | 493 | 0 |
| (5, 3, 3)(5) | 7 6 7 5 6<br>3 4 2 4 3<br>3 3 3 3 3 | 4 5 5 5 4<br>11 8 9 11 8 | 7285 | 203.92 | 432 | 23 | 23 | 1330 | 0.60 | 432 | 0 | 0 | 2494 | 6.37 | 488 | 37 | 532 | 0 |
| (5, 3, 3)(6) | 5 4 8 5 5<br>1 2 4 1 4<br>3 3 3 3 3 | 5 5 4 5 4<br>9 10 10 8 8 | 6885 | 216.11 | 419 | 15 | 19 | 1330 | 0.53 | 419 | 0 | 0 | 2372 | 6.20 | 477 | 35 | 512 | 0 |
| (5, 3, 3)(7) | 6 4 5 8 8<br>3 4 2 1 4<br>3 3 3 3 3 | 5 5 5 4 4<br>11 10 9 9 8 | 7205 | 217.19 | 427 | 21 | 32 | 1330 | 0.66 | 427 | 0 | 0 | 2470 | 6.27 | 462 | 37 | 509 | 0 |
| (5, 3, 3)(8) | 7 4 5 5 8<br>1 4 1 2 1<br>3 3 3 3 3 | 5 4 5 5 4<br>9 11 11 8 9 | 6965 | 186.32 | 430 | 17 | 25 | 1330 | 0.58 | 430 | 0 | 0 | 2399 | 6.34 | 464 | 35 | 512 | 0 |
| (5, 3, 3)(9) | 5 8 6 7 5<br>1 3 2 2 4<br>3 3 3 3 3 | 4 5 4 5 4<br>10 10 8 11 10 | 7165 | 221.54 | 429 | 17 | 26 | 1330 | 0.53 | 429 | 0 | 0 | 2459 | 6.30 | 483 | 36 | 511 | 0 |
| (5, 4, 1)(0) | 8 6 5 7 7<br>4 2 2 4 1<br>1 1 1 1 1 | 4 4 5 5 4<br>8 9 9 9 8<br>23 20 16 21 17 | 9925 | 989.07 | 453 | 36 | 40 | 1780 | 1.01 | 453 | 0 | 0 | 3408 | 8.89 | 634 | 51 | 739 | 0 |
| (5, 4, 1)(1) | 6 5 4 6 6<br>2 4 1 3 1<br>1 1 1 1 1 | 5 4 5 5 5<br>8 11 11 8 8<br>22 17 19 21 21 | 9925 | 617.96 | 439 | 33 | 33 | 1780 | 1.48 | 439 | 0 | 0 | 3416 | 8.48 | 596 | 51 | 746 | 0 |
| (5, 4, 1)(2) | 4 6 8 4 5<br>2 3 3 2 4<br>1 1 1 1 1 | 4 5 4 5 5<br>9 9 8 9 11<br>20 22 20 17 22 | 10045 | 653.13 | 442 | 39 | 45 | 1780 | 1.12 | 442 | 0 | 0 | 3452 | 8.56 | 574 | 51 | 701 | 0 |
| (5, 4, 1)(3) | 8 7 4 6 5<br>4 1 4 4 1<br>1 1 1 1 1 | 5 5 5 4 5<br>9 11 8 9 11<br>21 23 21 22 20 | 10525 | 532.44 | 459 | 42 | 54 | 1780 | 1.51 | 459 | 0 | 0 | 3605 | 8.96 | 624 | 54 | 776 | 0 |
| (5, 4, 1)(4) | 7 6 6 6 4<br>2 2 4 4 4<br>1 1 1 1 1 | 5 5 5 4 4<br>9 8 11 9 11<br>16 17 20 22 17 | 9925 | 234.74 | 441 | 39 | 39 | 1780 | 1.20 | 441 | 0 | 0 | 3409 | 8.79 | 615 | 51 | 717 | 0 |
| (5, 4, 1)(5) | 6 7 7 8 6<br>2 1 3 3 1<br>1 1 1 1 1 | 4 4 4 5 5<br>11 10 9 8 8<br>17 22 19 17 19 | 9845 | 649.71 | 447 | 29 | 29 | 1780 | 1.03 | 447 | 0 | 0 | 3384 | 8.44 | 611 | 50 | 708 | 0 |
| (5, 4, 1)(6) | 7 6 8 6 6<br>1 1 1 1 3<br>1 1 1 1 1 | 5 5 5 4 5<br>9 9 8 9 8<br>18 18 21 22 20 | 9845 | 657.29 | 433 | 32 | 32 | 1780 | 1.79 | 433 | 0 | 0 | 3388 | 8.68 | 613 | 50 | 756 | 0 |
| (5, 4, 1)(7) | 6 8 7 8 6<br>1 1 3 1 3<br>1 1 1 1 1 | 5 5 4 4 5<br>10 10 9 9 11<br>18 20 23 18 21 | 10245 | 830.76 | 451 | 31 | 31 | 1780 | 1.35 | 451 | 0 | 0 | 3514 | 8.95 | 643 | 52 | 741 | 0 |
| (5, 4, 1)(8) | 5 7 4 7 5<br>3 1 2 4 3<br>1 1 1 1 1 | 4 4 5 4 4<br>11 10 8 10 11<br>16 21 22 19 17 | 9885 | 791.38 | 464 | 31 | 36 | 1780 | 1.13 | 464 | 0 | 0 | 3400 | 8.45 | 597 | 51 | 720 | 0 |
| (5, 4, 1)(9) | 5 4 6 6 4<br>4 3 2 4 1<br>1 1 1 1 1 | 5 5 5 4 5<br>9 8 8 11 11<br>19 22 19 18 20 | 9925 | 502.06 | 432 | 35 | 39 | 1780 | 1.61 | 432 | 0 | 0 | 3415 | 8.34 | 620 | 51 | 713 | 0 |
| (5, 4, 3)(0) | 7 6 8 4 5<br>4 1 4 1 3<br>3 3 3 3 3 | 4 4 4 5 4<br>10 9 11 10 10<br>23 20 20 17 18 | 11085 | 348.21 | 541 | 66 | 66 | 1780 | 1.45 | 541 | 0 | 0 | 4003 | 10.34 | 761 | 60 | 843 | 0 |
| (5, 4, 3)(1) | 4 8 8 6 5<br>3 4 3 2 3<br>3 3 3 3 3 | 5 5 4 4 5<br>9 9 11 11 9<br>23 18 21 17 16 | 11125 | 335.71 | 555 | 110 | 114 | 1780 | 2.09 | 555 | 0 | 0 | 4013 | 10.55 | 791 | 60 | 945 | 0 |
| (5, 4, 3)(2) | 5 5 7 8 5<br>4 2 4 3 2<br>3 3 3 3 3 | 5 4 5 5 4<br>9 8 11 11 8<br>17 22 23 21 22 | 11365 | 533.02 | 564 | 73 | 131 | 1780 | 1.41 | 564 | 0 | 0 | 4105 | 40.32 | 677 | 61 | 992 | 0 |
| (5, 4, 3)(3) | 8 4 7 5 5<br>1 3 1 4 4<br>3 3 3 3 3 | 4 4 4 5 4<br>8 9 8 10 10<br>17 18 19 16 16 | 10445 | 255.76 | 522 | 92 | 93 | 1780 | 1.69 | 522 | 0 | 0 | 3770 | 9.59 | 718 | 56 | 860 | 0 |
| (5, 4, 3)(4) | 7 6 8 7 8<br>4 2 4 1 4<br>3 3 3 3 3 | 4 4 4 5 4<br>9 8 10 9 8<br>19 16 22 23 19 | 11165 | 242.35 | 542 | 65 | 96 | 1780 | 1.58 | 542 | 0 | 0 | 4034 | 10.71 | 762 | 60 | 906 | 0 |
| (5, 4, 3)(5) | 6 4 5 6 4<br>1 3 3 4 3<br>3 3 3 3 3 | 5 5 5 4 5<br>11 9 10 10 8<br>22 18 18 19 23 | 11045 | 289.41 | 556 | 52 | 109 | 1780 | 1.51 | 556 | 0 | 0 | 3994 | 10.68 | 761 | 59 | 11016 | 1 |
| (5, 4, 3)(6) | 5 5 4 4 4<br>4 3 3 3 3<br>3 3 3 3 3 | 4 5 4 5 5<br>11 8 11 8 9<br>20 20 20 21 17 | 10845 | 347.71 | 548 | 72 | 108 | 1780 | 2.55 | 548 | 0 | 0 | 3930 | 9.99 | 716 | 58 | 865 | 0 |
| (5, 4, 3)(7) | 6 7 8 8 8<br>1 1 1 1 2<br>3 3 3 3 3 | 5 5 5 4 5<br>8 9 11 11 10<br>18 17 16 22 17 | 10845 | 275.29 | 548 | 62 | 95 | 1780 | 1.93 | 548 | 0 | 0 | 3925 | 9.94 | 738 | 58 | 849 | 0 |
| (5, 4, 3)(8) | 8 5 8 7 7<br>4 4 2 4 1<br>3 3 3 3 3 | 5 4 5 5 5<br>9 10 11 8 8<br>21 20 17 18 20 | 11205 | 361.93 | 558 | 72 | 100 | 1780 | 1.84 | 558 | 0 | 0 | 4048 | 10.96 | 778 | 60 | 30688 | 1 |
| (5, 4, 3)(9) | 6 8 5 7 5<br>1 2 4 3 4<br>3 3 3 3 3 | 5 5 4 5 5<br>10 10 11 11 10<br>19 23 17 22 19 | 11405 | 353.47 | 567 | 76 | 111 | 1780 | 1.78 | 567 | 0 | 0 | 4118 | 40.35 | 735 | 61 | 837 | 0 |
| (6, 3, 1)(0) | 4 6 4 7 5 5<br>2 1 4 1 4 1<br>1 1 1 1 1 1 | 4 5 5 5 5 4<br>10 11 11 9 10 11 | 8454 | 910.78 | 416 | 19 | 24 | 1980 | 1.66 | 416 | 0 | 0 | 2994 | 7.22 | 544 | 44 | 615 | 0 |
| (6, 3, 1)(1) | 4 6 6 4 5 4<br>3 2 1 1 4 3<br>1 1 1 1 1 1 | 4 4 5 5 5 4<br>9 11 11 8 9 9 | 8118 | 1049.49 | 412 | 14 | 14 | 1980 | 1.38 | 412 | 0 | 0 | 2883 | 6.90 | 519 | 43 | 614 | 0 |
| (6, 3, 1)(2) | 7 6 4 5 6 6<br>2 3 4 2 2 4<br>1 1 1 1 1 1 | 5 5 5 4 4 4<br>10 11 10 10 11 8 | 8646 | 714.10 | 430 | 23 | 23 | 1980 | 1.66 | 430 | 0 | 0 | 3051 | 7.29 | 552 | 45 | 630 | 0 |
| (6, 3, 1)(3) | 4 5 6 6 4 5<br>4 4 2 4 2 2<br>1 1 1 1 1 1 | 5 5 5 4 5 4<br>9 11 11 11 11 9 | 8646 | 867.76 | 437 | 17 | 31 | 1980 | 2.30 | 437 | 0 | 0 | 3054 | 7.63 | 560 | 45 | 623 | 0 |
| (6, 3, 1)(4) | 5 4 8 8 7 4<br>2 4 1 3 2 2<br>1 1 1 1 1 1 | 4 4 5 5 5 5<br>8 9 11 8 8 10 | 8358 | 1184.06 | 421 | 18 | 18 | 1980 | 3.50 | 421 | 0 | 0 | 2956 | 7.15 | 556 | 44 | 632 | 0 |
| (6, 3, 1)(5) | 4 4 4 4 6 7<br>2 4 3 2 1 4<br>1 1 1 1 1 1 | 5 4 5 4 5 4<br>11 8 9 8 9 8 | 8022 | 3600.19 | 426 | 18 | 18 | 1980 | 1.88 | 426 | 0 | 0 | 2849 | 6.87 | 536 | 42 | 599 | 0 |
| (6, 3, 1)(6) | 4 5 5 7 6 5<br>4 2 4 3 3 4<br>1 1 1 1 1 1 | 4 5 4 5 4 4<br>8 10 8 11 10 11 | 8550 | 1888.13 | 438 | 25 | 25 | 1980 | 1.42 | 438 | 0 | 0 | 3018 | 7.67 | 574 | 45 | 565 | 0 |
| (6, 3, 1)(7) | 7 8 6 8 6 4<br>4 1 4 2 3 1<br>1 1 1 1 1 1 | 4 4 5 5 4 5<br>10 10 11 11 9 9 | 8790 | 2129.50 | 440 | 16 | 35 | 1980 | 1.53 | 440 | 0 | 0 | 3096 | 7.64 | 540 | 46 | 670 | 0 |
| (6, 3, 1)(8) | 5 4 5 8 6 6<br>3 2 1 4 4 3<br>1 1 1 1 1 1 | 5 5 5 4 5 4<br>9 10 9 8 11 10 | 8550 | 1188.69 | 431 | 20 | 30 | 1980 | 2.41 | 431 | 0 | 0 | 3019 | 7.28 | 518 | 45 | 593 | 0 |
| (6, 3, 1)(9) | 7 5 4 6 4 6<br>2 3 1 4 1 1<br>1 1 1 1 1 1 | 4 5 4 4 5 5<br>9 9 9 9 10 11 | 8166 | 764.47 | 403 | 19 | 19 | 1980 | 1.56 | 403 | 0 | 0 | 2898 | 7.01 | 515 | 43 | 619 | 0 |
| (6, 3, 3)(0) | 4 7 5 6 5 4<br>3 2 3 3 3 1<br>3 3 3 3 3 3 | 4 5 4 4 5 4<br>9 8 11 11 8 11 | 9990 | 1491.13 | 579 | 27 | 27 | 1980 | 1.61 | 579 | 0 | 0 | 3528 | 8.60 | 685 | 52 | 730 | 0 |
| (6, 3, 3)(1) | 5 8 5 6 7 8<br>4 2 3 1 3 1<br>3 3 3 3 3 3 | 5 5 5 5 4 5<br>9 10 10 8 9 11 | 9942 | 1522.60 | 593 | 31 | 32 | 1980 | 2.60 | 593 | 0 | 0 | 3665 | 9.30 | 703 | 54 | 752 | 0 |
| (6, 3, 3)(2) | 4 7 4 7 7 4<br>4 2 2 3 1 4<br>3 3 3 3 3 3 | 5 5 4 4 5 5<br>10 8 10 10 8 9 | 9606 | 557.10 | 589 | 29 | 48 | 1980 | 2.58 | 589 | 0 | 1 | 3557 | 8.95 | 654 | 53 | 731 | 0 |
| (6, 3, 3)(3) | 5 6 6 6 7 8<br>1 1 3 1 2 4<br>3 3 3 3 3 3 | 4 4 5 4 4 5<br>9 11 10 8 10 11 | 9750 | 3600.29 | 588 | 30 | 44 | 1980 | 2.92 | 588 | 0 | 0 | 3604 | 8.88 | 681 | 54 | 742 | 0 |
| (6, 3, 3)(4) | 5 8 6 5 5 7<br>1 4 4 1 1 3<br>3 3 3 3 3 3 | 4 5 5 5 4 4<br>8 8 11 10 8 8 | 9510 | 2719.56 | 563 | 48 | 48 | 1980 | 2.75 | 563 | 0 | 0 | 3524 | 8.62 | 671 | 52 | 670 | 0 |
| (6, 3, 3)(5) | 8 6 6 8 8 7<br>4 1 2 4 2 4<br>3 3 3 3 3 3 | 4 5 5 4 4 5<br>10 10 11 10 10 10 | 10326 | 1694.36 | 617 | 32 | 34 | 1980 | 2.25 | 617 | 0 | 0 | 3802 | 9.47 | 690 | 57 | 789 | 0 |
| (6, 3, 3)(6) | 7 7 6 8 6 8<br>4 3 1 4 3 3<br>3 3 3 3 3 3 | 5 4 4 5 5 5<br>11 10 11 11 8 11 | 10374 | 1480.06 | 604 | 34 | 55 | 1980 | 2.50 | 604 | 0 | 1 | 3834 | 9.34 | 680 | 57 | 794 | 0 |
| (6, 3, 3)(7) | 4 4 8 4 8 4<br>4 4 2 3 2 2<br>3 3 3 3 3 3 | 5 4 4 4 5 4<br>8 8 11 10 10 9 | 9558 | 805.97 | 580 | 31 | 31 | 1980 | 2.04 | 580 | 0 | 0 | 3541 | 8.90 | 645 | 53 | 669 | 0 |
| (6, 3, 3)(8) | 6 5 5 8 6 7<br>1 3 3 2 4 2<br>3 3 3 3 3 3 | 4 4 4 4 5 5<br>11 8 8 11 9 9 | 9702 | 1270.44 | 586 | 28 | 28 | 1980 | 1.95 | 586 | 0 | 0 | 3586 | 9.04 | 680 | 53 | 732 | 0 |
| (6, 3, 3)(9) | 5 4 7 6 7 5<br>2 2 2 4 4 1<br>3 3 3 3 3 3 | 5 5 4 4 5 5<br>9 10 8 9 8 10 | 9558 | 1451.40 | 594 | 24 | 46 | 1980 | 1.90 | 594 | 0 | 0 | 3541 | 8.81 | 647 | 53 | 752 | 0 |
| (6, 4, 1)(0) | 8 5 6 5 8 8<br>3 2 1 2 1 2<br>1 1 1 1 1 1 | 4 4 5 4 4 5<br>9 9 9 11 11 8<br>17 18 16 18 18 22 | 13974 | 3404.77 | 579 | 99 | 157 | 2652 | 3.75 | 579 | 0 | 0 | 4935 | 41.81 | 865 | 74 | 1033 | 0 |
| (6, 4, 1)(1) | 5 7 6 5 4 7<br>1 4 2 1 2 3<br>1 1 1 1 1 1 | 4 4 5 4 4 5<br>9 11 10 10 11 10<br>17 22 20 18 21 16 | 14214 | 3600.65 | 590 | 67 | 67 | 2652 | 2.50 | 590 | 0 | 1 | 5019 | 41.73 | 891 | 75 | 1095 | 0 |
| (6, 4, 1)(2) | 4 5 7 6 8 4<br>4 4 2 4 2 4<br>1 1 1 1 1 1 | 5 4 4 4 4 5<br>10 10 11 10 11 9<br>22 16 23 20 16 17 | 13878 | 3600.61 | 631 | 178 | 200 | 2652 | 5.69 | 631 | 0 | 1 | 5124 | 42.51 | 877 | 76 | 1077 | 0 |
| (6, 4, 1)(3) | 8 8 5 5 8 6<br>4 1 4 3 3 2<br>1 1 1 1 1 1 | 4 4 4 4 4 4<br>8 11 9 10 8 11<br>21 19 22 21 22 23 | 14358 | 3600.65 | 659 | 110 | 193 | 2652 | 4.44 | 659 | 0 | 2 | 5297 | 43.79 | 873 | 79 | 1218 | 0 |
| (6, 4, 1)(4) | 6 7 8 6 6 7<br>4 2 3 4 4 1<br>1 1 1 1 1 1 | 5 4 5 4 5 4<br>11 9 8 11 8 9<br>21 17 17 18 20 20 | 13830 | 3600.67 | 614 | 114 | 114 | 2652 | 4.58 | 614 | 0 | 0 | 5104 | 42.49 | 924 | 76 | 1010 | 0 |
| (6, 4, 1)(5) | 7 7 5 7 8 6<br>4 3 1 1 4 4<br>1 1 1 1 1 1 | 4 4 5 5 4 5<br>8 11 10 11 10 11<br>19 22 17 19 22 19 | 14262 | 2958.23 | 605 | 134 | 205 | 2652 | 9.59 | 605 | 1 | 2 | 5249 | 42.95 | 844 | 78 | 1031 | 0 |
| (6, 4, 1)(6) | 5 4 7 6 8 5<br>4 4 3 3 1 4<br>1 1 1 1 1 1 | 4 4 4 4 4 5<br>10 11 11 11 9 9<br>21 16 20 22 17 23 | 14070 | 3600.51 | 618 | 108 | 195 | 2652 | 3.78 | 618 | 0 | 1 | 5188 | 43.47 | 893 | 77 | 1069 | 0 |
| (6, 4, 1)(7) | 7 4 8 7 6 6<br>3 1 3 4 1 2<br>1 1 1 1 1 1 | 5 5 5 5 4 5<br>8 8 10 9 10 10<br>20 17 16 18 20 22 | 13638 | 3600.54 | 596 | 63 | 63 | 2652 | 14.36 | 591 | 1 | 2 | 5030 | 41.90 | 927 | 75 | 992 | 0 |
| (6, 4, 1)(8) | 8 4 8 7 6 4<br>2 2 2 2 2 2<br>1 1 1 1 1 1 | 5 4 5 4 4 4<br>8 11 10 9 11 10<br>19 17 19 17 23 16 | 13446 | 3600.46 | 595 | 97 | 179 | 2652 | 7.55 | 589 | 0 | 1 | 4969 | 42.17 | 874 | 74 | 1030 | 0 |
| (6, 4, 1)(9) | 6 6 8 4 8 4<br>1 3 2 4 1 4<br>1 1 1 1 1 1 | 5 5 5 4 5 4<br>8 11 8 10 9 10<br>16 22 18 17 22 21 | 13734 | 1750.94 | 575 | 112 | 168 | 2652 | 8.40 | 575 | 0 | 1 | 5063 | 42.25 | 909 | 75 | 1129 | 0 |
| (6, 4, 3)(0) | 5 8 6 6 5 5<br>4 2 1 4 4 3<br>3 3 3 3 3 3 | 4 5 5 5 4 5<br>9 11 10 10 11 9<br>21 22 22 22 16 23 | 16470 | 1525.45 | 785 | 270 | 463 | 2652 | 3.52 | 785 | 0 | 1 | 6109 | 79.19 | 1012 | 91 | 11313 | 1 |
| (6, 4, 3)(1) | 8 6 4 8 5 5<br>3 1 3 1 3 4<br>3 3 3 3 3 3 | 4 4 4 5 4 5<br>10 8 8 8 9 10<br>19 21 21 20 21 18 | 15750 | 775.94 | 742 | 270 | 286 | 2652 | 4.17 | 742 | 0 | 1 | 5839 | 45.83 | 1011 | 87 | 1388 | 0 |
| (6, 4, 3)(2) | 4 5 8 7 5 7<br>2 3 3 4 4 2<br>3 3 3 3 3 3 | 5 5 5 4 4 5<br>11 10 10 11 9 8<br>17 21 21 22 20 22 | 16374 | 1350.54 | 765 | 424 | 424 | 2652 | 4.36 | 765 | 0 | 1 | 6060 | 78.41 | 1056 | 90 | 1375 | 0 |
| (6, 4, 3)(3) | 7 6 6 6 7 8<br>3 2 2 2 3 3<br>3 3 3 3 3 3 | 5 5 5 4 5 5<br>10 10 10 11 9 11<br>23 18 22 21 18 18 | 16422 | 1538.81 | 762 | 414 | 414 | 2652 | 4.10 | 762 | 0 | 0 | 6075 | 78.13 | 1077 | 91 | 1449 | 0 |
| (6, 4, 3)(4) | 4 8 4 6 8 7<br>4 3 1 2 2 1<br>3 3 3 3 3 3 | 5 5 5 4 4 5<br>11 11 11 10 9 11<br>17 17 20 17 22 20 | 15942 | 1164.22 | 751 | 210 | 317 | 2652 | 3.80 | 751 | 0 | 1 | 5904 | 45.80 | 977 | 88 | 16306 | 1 |
| (6, 4, 3)(5) | 7 4 6 4 5 5<br>1 4 3 3 1 4<br>3 3 3 3 3 3 | 4 5 4 4 5 5<br>8 8 8 9 11 10<br>19 16 19 21 21 22 | 15558 | 729.09 | 735 | 252 | 261 | 2652 | 5.09 | 735 | 0 | 1 | 5779 | 45.73 | 1067 | 86 | 1303 | 0 |
| (6, 4, 3)(6) | 6 8 7 6 5 7<br>3 4 3 2 2 3<br>3 3 3 3 3 3 | 4 4 4 5 5 5<br>10 8 11 9 10 11<br>16 19 21 22 20 17 | 16038 | 1129.19 | 739 | 388 | 388 | 2652 | 4.40 | 739 | 0 | 1 | 5946 | 46.46 | 1028 | 89 | 1301 | 0 |
| (6, 4, 3)(7) | 4 5 8 4 8 8<br>1 3 1 3 2 3<br>3 3 3 3 3 3 | 4 5 5 5 4 4<br>10 8 10 11 10 11<br>21 21 17 19 19 23 | 16038 | 992.33 | 739 | 322 | 388 | 2652 | 3.98 | 739 | 0 | 1 | 5952 | 45.32 | 1037 | 89 | 1536 | 0 |
| (6, 4, 3)(8) | 4 6 7 8 5 8<br>2 4 1 2 3 4<br>3 3 3 3 3 3 | 5 5 5 4 5 4<br>10 9 10 11 8 10<br>22 23 20 20 21 18 | 16374 | 1387.26 | 771 | 426 | 426 | 2652 | 4.05 | 771 | 0 | 1 | 6060 | 78.82 | 1063 | 90 | 1258 | 0 |
| (6, 4, 3)(9) | 5 4 7 4 8 6<br>3 1 3 1 3 1<br>3 3 3 3 3 3 | 4 4 4 4 5 4<br>9 9 11 9 10 11<br>23 21 21 21 22 22 | 16182 | 3600.29 | 768 | 447 | 483 | 2652 | 5.39 | 768 | 0 | 2 | 6004 | 77.47 | 997 | 90 | 1427 | 0 |
| (7, 3, 1)(0) | 6 4 4 8 6 8 6<br>3 1 3 2 3 3 4<br>1 1 1 1 1 1 1 | 5 4 4 5 5 5 5<br>11 11 11 8 8 9 11 | 11431 | 3600.32 | 564 | 48 | 92 | 2758 | 40.65 | 548 | 0 | 3 | 4268 | 39.49 | 716 | 64 | 868 | 0 |
| (7, 3, 1)(1) | 8 4 5 8 5 4 6<br>2 3 1 1 3 4 1<br>1 1 1 1 1 1 1 | 5 4 4 4 5 4 5<br>10 8 8 10 9 11 8 | 10759 | 3600.10 | 550 | 21 | 33 | 2758 | 19.42 | 550 | 0 | 1 | 4027 | 9.27 | 705 | 60 | 829 | 0 |
| (7, 3, 1)(2) | 6 4 7 4 5 7 5<br>3 3 3 2 4 4 2<br>1 1 1 1 1 1 1 | 4 4 5 4 5 5 4<br>11 10 11 11 8 10 9 | 11263 | 3600.32 | 572 | 49 | 49 | 2758 | 13.28 | 562 | 0 | 2 | 4213 | 39.53 | 740 | 63 | 833 | 0 |
| (7, 3, 1)(3) | 5 8 4 4 4 5 5<br>4 2 4 2 2 2 3<br>1 1 1 1 1 1 1 | 4 5 4 5 4 5 5<br>10 8 8 8 10 9 11 | 10759 | 1996.10 | 538 | 21 | 41 | 2758 | 28.35 | 538 | 0 | 4 | 4028 | 9.63 | 630 | 60 | 828 | 0 |
| (7, 3, 1)(4) | 6 8 5 6 8 5 7<br>4 1 2 4 2 1 3<br>1 1 1 1 1 1 1 | 4 4 4 5 5 4 5<br>11 9 9 10 8 10 11 | 11319 | 3600.27 | 565 | 28 | 46 | 2758 | 25.30 | 564 | 0 | 1 | 4229 | 39.10 | 729 | 63 | 859 | 0 |
| (7, 3, 1)(5) | 6 6 4 5 8 7 7<br>1 4 1 2 4 4 1<br>1 1 1 1 1 1 1 | 4 4 4 4 4 5 5<br>9 10 8 9 8 8 8 | 10759 | 3600.24 | 540 | 22 | 34 | 2758 | 5.59 | 540 | 0 | 1 | 4022 | 9.40 | 717 | 60 | 802 | 0 |
| (7, 3, 1)(6) | 7 4 4 5 7 5 4<br>4 3 2 4 1 1 2<br>1 1 1 1 1 1 1 | 4 4 5 4 4 5 5<br>9 11 8 8 11 11 11 | 10927 | 3600.23 | 578 | 94 | 98 | 2758 | 13.37 | 567 | 0 | 1 | 4086 | 9.67 | 732 | 61 | 840 | 0 |
| (7, 3, 1)(7) | 6 6 4 8 6 7 7<br>2 1 4 1 3 3 2<br>1 1 1 1 1 1 1 | 5 5 5 5 5 4 4<br>10 8 10 10 10 9 10 | 11263 | 3600.04 | 570 | 30 | 49 | 2758 | 196.39 | 563 | 0 | 1 | 4212 | 39.24 | 693 | 63 | 855 | 0 |
| (7, 3, 1)(8) | 5 6 5 7 5 8 4<br>3 2 1 3 2 4 2<br>1 1 1 1 1 1 1 | 5 4 4 5 5 5 4<br>11 11 9 9 9 8 8 | 10983 | 3600.30 | 542 | 28 | 49 | 2758 | 16.05 | 537 | 0 | 1 | 4101 | 39.16 | 696 | 61 | 826 | 0 |
| (7, 3, 1)(9) | 6 5 7 5 5 7 5<br>4 4 1 1 3 4 1<br>1 1 1 1 1 1 1 | 4 4 4 4 5 5 5<br>10 11 11 8 8 8 10 | 11039 | 3600.05 | 549 | 96 | 118 | 2758 | 10.81 | 547 | 0 | 2 | 4119 | 38.65 | 711 | 61 | 869 | 0 |
| (7, 3, 3)(0) | 7 6 5 8 7 5 4<br>2 1 2 4 1 4 1<br>3 3 3 3 3 3 3 | 4 5 5 5 4 4 4<br>9 11 8 8 8 8 8 | 12775 | 3600.40 | 746 | 48 | 48 | 2758 | 6.16 | 746 | 0 | 1 | 4813 | 41.64 | 860 | 72 | 942 | 0 |
| (7, 3, 3)(1) | 8 5 6 7 6 6 5<br>3 2 3 2 3 1 1<br>3 3 3 3 3 3 3 | 5 4 4 5 5 5 4<br>8 11 9 10 9 11 8 | 13167 | 3600.38 | 763 | 53 | 203 | 2758 | 5.67 | 763 | 0 | 1 | 4964 | 42.08 | 864 | 74 | 1017 | 0 |
| (7, 3, 3)(2) | 5 4 5 7 7 8 6<br>3 2 4 3 2 2 1<br>3 3 3 3 3 3 3 | 5 5 5 4 4 5 5<br>8 11 9 8 9 11 8 | 13167 | 3600.08 | 772 | 53 | 53 | 2758 | 6.16 | 772 | 0 | 1 | 4963 | 41.65 | 898 | 74 | 1031 | 0 |
| (7, 3, 3)(3) | 4 6 8 7 4 4 6<br>1 3 2 4 2 3 1<br>3 3 3 3 3 3 3 | 4 5 4 5 4 4 4<br>8 8 9 8 10 8 8 | 12607 | 3600.30 | 732 | 33 | 33 | 2758 | 6.85 | 732 | 1 | 1 | 4739 | 41.19 | 844 | 71 | 900 | 0 |
| (7, 3, 3)(4) | 8 5 4 8 7 8 6<br>1 2 2 2 4 4 1<br>3 3 3 3 3 3 3 | 4 5 4 5 4 4 4<br>8 8 10 11 9 10 9 | 13223 | 3600.34 | 773 | 45 | 119 | 2758 | 7.27 | 773 | 0 | 1 | 4979 | 41.40 | 849 | 74 | 956 | 0 |
| (7, 3, 3)(5) | 4 7 6 7 7 6 4<br>4 3 4 4 3 3 2<br>3 3 3 3 3 3 3 | 4 4 5 5 4 5 5<br>8 9 9 11 10 9 8 | 13391 | 3600.36 | 757 | 43 | 114 | 2758 | 6.88 | 757 | 0 | 1 | 5034 | 41.82 | 835 | 75 | 1054 | 0 |
| (7, 3, 3)(6) | 8 7 8 5 8 6 6<br>2 3 4 2 2 4 2<br>3 3 3 3 3 3 3 | 4 4 5 5 5 4 4<br>11 8 9 8 8 11 8 | 13447 | 3600.35 | 772 | 44 | 63 | 2758 | 5.93 | 772 | 0 | 1 | 5050 | 41.66 | 884 | 75 | 1054 | 0 |
| (7, 3, 3)(7) | 7 7 6 7 8 5 8<br>4 2 3 1 4 3 1<br>3 3 3 3 3 3 3 | 5 5 5 4 5 4 4<br>8 11 10 11 8 9 11 | 13671 | 3600.45 | 804 | 46 | 54 | 2758 | 7.42 | 795 | 0 | 1 | 5146 | 41.96 | 904 | 77 | 1089 | 0 |
| (7, 3, 3)(8) | 8 8 5 7 5 7 5<br>3 1 1 3 2 3 1<br>3 3 3 3 3 3 3 | 4 5 5 4 4 4 4<br>9 10 9 11 9 11 8 | 13167 | 3600.35 | 772 | 42 | 56 | 2758 | 7.18 | 766 | 0 | 2 | 4963 | 42.11 | 879 | 74 | 1027 | 0 |
| (7, 3, 3)(9) | 8 4 5 6 7 5 6<br>3 1 4 3 1 2 3<br>3 3 3 3 3 3 3 | 4 4 4 4 5 4 4<br>10 11 9 8 11 10 10 | 13167 | 3600.37 | 765 | 80 | 208 | 2758 | 5.78 | 765 | 0 | 1 | 4964 | 41.52 | 809 | 74 | 986 | 0 |
| (7, 4, 1)(0) | 6 4 4 5 7 8 7<br>4 4 4 1 2 2 3<br>1 1 1 1 1 1 1 | 5 4 4 4 4 5 4<br>10 11 11 11 9 10 9<br>19 19 16 17 19 23 21 | 18823 | 3600.37 | 785 | 170 | 373 | 3696 | 17.51 | 782 | 0 | 5 | 7075 | 80.94 | 1109 | 100 | 11805 | 1 |
| (7, 4, 1)(1) | 8 7 5 7 5 6 5<br>4 4 1 4 1 1 3<br>1 1 1 1 1 1 1 | 4 4 4 4 4 5 5<br>9 11 9 10 9 9 11<br>20 18 17 22 18 20 19 | 18655 | 3600.13 | 753 | 325 | 368 | 3696 | 17.60 | 748 | 3 | 3 | 7018 | 81.03 | 1093 | 100 | 1287 | 0 |
| (7, 4, 1)(2) | 6 5 4 7 7 6 6<br>4 3 3 3 4 3 2<br>1 1 1 1 1 1 1 | 5 4 4 4 5 5 4<br>10 11 9 8 9 8 10<br>19 23 19 18 23 21 17 | 18991 | 3600.12 | 791 | 148 | 215 | 3696 | 20.19 | 791 | 0 | 3 | 7130 | 81.24 | 1172 | 100 | 11635 | 1 |
| (7, 4, 1)(3) | 6 8 4 6 8 7 4<br>2 1 4 3 1 3 4<br>1 1 1 1 1 1 1 | 5 4 5 5 5 4 5<br>11 9 11 9 8 10 8<br>21 23 16 21 19 18 19 | 18879 | 3600.33 | 793 | 202 | 366 | 3696 | 46.11 | 773 | 0 | 3 | 7094 | 81.55 | 1157 | 100 | 1526 | 0 |
| (7, 4, 1)(4) | 4 7 7 4 4 7 6<br>2 4 3 2 4 1 3<br>1 1 1 1 1 1 1 | 4 5 4 5 5 4 4<br>8 10 10 11 10 10 9<br>20 19 19 16 23 16 16 | 18319 | 3600.13 | 797 | 184 | 351 | 3696 | 29.04 | 771 | 0 | 5 | 6888 | 80.96 | 1138 | 100 | 1610 | 0 |
| (7, 4, 1)(5) | 6 5 8 8 6 6 8<br>4 1 3 2 1 2 4<br>1 1 1 1 1 1 1 | 4 4 4 4 5 4 4<br>8 8 11 10 8 8 10<br>17 16 21 16 17 19 19 | 18095 | 3600.13 | 762 | 277 | 284 | 3696 | 15.28 | 757 | 0 | 3 | 6787 | 79.21 | 1132 | 100 | 1609 | 0 |
| (7, 4, 1)(6) | 7 4 5 8 6 5 5<br>1 2 4 4 4 4 2<br>1 1 1 1 1 1 1 | 5 4 4 4 5 4 4<br>11 10 8 9 10 8 9<br>16 18 19 19 17 23 23 | 18599 | 3600.32 | 807 | 143 | 189 | 3696 | 13.80 | 791 | 0 | 4 | 6980 | 79.96 | 1061 | 100 | 1793 | 0 |
| (7, 4, 1)(7) | 6 4 7 8 4 4 8<br>3 1 2 4 2 1 1<br>1 1 1 1 1 1 1 | 5 4 4 5 4 5 4<br>10 8 11 9 9 11 9<br>19 18 18 21 23 16 19 | 18375 | 3600.23 | 778 | 298 | 325 | 3696 | 26.04 | 757 | 0 | 5 | 6910 | 81.75 | 1133 | 100 | 1462 | 0 |
| (7, 4, 1)(8) | 4 8 5 5 6 8 6<br>1 1 3 1 1 3 3<br>1 1 1 1 1 1 1 | 5 4 4 5 4 4 4<br>9 10 8 10 10 11 9<br>23 17 21 18 22 22 21 | 18823 | 3600.15 | 765 | 146 | 388 | 3696 | 19.47 | 765 | 0 | 2 | 7081 | 81.04 | 1127 | 100 | 16513 | 1 |
| (7, 4, 1)(9) | 7 5 6 6 6 4 4<br>1 4 2 3 1 3 3<br>1 1 1 1 1 1 1 | 4 4 4 4 5 4 4<br>9 10 9 9 8 11 11<br>19 22 16 19 20 16 20 | 18151 | 3600.18 | 771 | 130 | 299 | 3696 | 15.25 | 767 | 0 | 3 | 6834 | 80.83 | 1087 | 100 | 11386 | 1 |
| (7, 4, 3)(0) | 5 4 7 7 4 7 4<br>1 1 2 2 1 4 1<br>3 3 3 3 3 3 3 | 5 4 5 4 5 5 4<br>11 11 8 11 9 9 11<br>19 18 22 17 17 16 20 | 20895 | 3600.78 | 952 | 592 | 765 | 3696 | 17.00 | 951 | 0 | 2 | 7893 | 85.48 | 1270 | 100 | 41361 | 2 |
| (7, 4, 3)(2) | 7 4 7 7 5 6 5<br>2 3 3 1 1 1 1<br>3 3 3 3 3 3 3 | 5 5 5 5 5 5 4<br>8 10 9 11 9 11 9<br>23 23 17 16 20 17 21 | 21399 | 3600.16 | 959 | 670 | 786 | 3696 | 10.98 | 959 | 0 | 2 | 8080 | 86.14 | 1359 | 100 | 1791 | 0 |
| (7, 4, 3)(3) | 4 8 7 4 8 5 7<br>4 1 3 3 4 1 4<br>3 3 3 3 3 3 3 | 5 5 5 5 5 5 4<br>8 11 8 8 10 8 9<br>22 16 16 17 19 19 19 | 21175 | 3538.95 | 931 | 741 | 810 | 3696 | 13.82 | 931 | 0 | 3 | 7994 | 85.19 | 1397 | 100 | 1744 | 0 |
| (7, 4, 3)(4) | 6 4 6 7 5 6 4<br>3 2 1 1 3 3 4<br>3 3 3 3 3 3 3 | 4 5 5 5 4 5 5<br>8 8 8 9 9 8 8<br>23 20 20 21 16 22 23 | 21399 | 2803.23 | 967 | 520 | 693 | 3696 | 15.47 | 967 | 0 | 3 | 8078 | 87.07 | 1262 | 100 | 31435 | 1 |
| (7, 4, 3)(5) | 6 4 5 5 5 7 4<br>3 4 2 3 3 3 1<br>3 3 3 3 3 3 3 | 5 5 5 4 4 4 4<br>10 10 10 8 8 11 11<br>23 16 17 17 17 18 18 | 20839 | 3600.25 | 949 | 451 | 648 | 3696 | 16.61 | 933 | 0 | 4 | 7869 | 85.58 | 1304 | 100 | 16860 | 1 |
| (7, 4, 3)(6) | 5 4 6 7 7 4 4<br>4 2 2 2 1 2 1<br>3 3 3 3 3 3 3 | 4 5 5 4 5 5 5<br>9 11 11 10 10 11 8<br>17 17 20 23 16 16 21 | 21063 | 3521.01 | 961 | 806 | 835 | 3696 | 11.60 | 961 | 0 | 3 | 7949 | 85.44 | 1328 | 100 | 26763 | 2 |
| (8, 3, 1)(0) | 7 4 4 7 5 6 8 7<br>1 2 1 2 2 1 4 1<br>1 1 1 1 1 1 1 1 | 5 5 5 5 4 5 5 5<br>9 9 9 9 10 11 8 9 | 14280 | 3600.07 | 698 | 464 | 464 | 3664 | 1630.29 | 679 | 0 | 3 | 5412 | 41.85 | 943 | 81 | 1117 | 0 |
| (8, 3, 1)(1) | 4 4 4 6 5 4 4 8<br>2 3 4 3 2 1 3 4<br>1 1 1 1 1 1 1 1 | 4 4 4 4 4 5 5 4<br>8 11 10 9 9 11 8 9 | 13960 | 3600.08 | 743 | 254 | 254 | 3664 | 102.66 | 743 | 0 | 1 | 5303 | 42.27 | 969 | 79 | 1092 | 0 |
| (8, 3, 1)(2) | 6 4 7 6 4 6 8 4<br>3 1 3 3 2 3 4 3<br>1 1 1 1 1 1 1 1 | 5 4 5 4 5 4 4 4<br>11 11 8 9 8 11 10 8 | 14408 | 3600.07 | 720 | 271 | 272 | 3664 | 85.87 | 710 | 0 | 2 | 5473 | 43.18 | 994 | 82 | 1175 | 0 |
| (8, 3, 1)(3) | 8 8 4 5 7 8 7 6<br>3 3 3 1 2 1 2 4<br>1 1 1 1 1 1 1 1 | 4 4 5 5 5 4 5 5<br>10 10 11 11 11 8 9 8 | 14984 | 3600.09 | 754 | 407 | 480 | 3664 | 716.71 | 716 | 0 | 3 | 5666 | 44.02 | 938 | 84 | 1140 | 0 |
| (8, 3, 1)(4) | 6 6 6 8 7 5 6 7<br>1 4 2 3 3 3 1 2<br>1 1 1 1 1 1 1 1 | 4 4 5 5 5 5 5 5<br>10 10 10 9 10 11 10 10 | 14984 | 3600.10 | 731 | 327 | 348 | 3664 | 2959.87 | 721 | 0 | 5 | 5690 | 43.04 | 902 | 85 | 1134 | 0 |
| (8, 3, 1)(5) | 6 7 8 6 5 5 6 6<br>4 2 3 1 1 2 3 2<br>1 1 1 1 1 1 1 1 | 4 5 4 5 5 5 4 4<br>10 9 11 10 9 8 10 10 | 14536 | 3600.07 | 722 | 304 | 314 | 3664 | 289.63 | 709 | 0 | 3 | 5517 | 42.54 | 925 | 82 | 1082 | 0 |
| (8, 3, 1)(6) | 5 7 4 7 7 6 4 5<br>2 1 1 2 3 3 2 2<br>1 1 1 1 1 1 1 1 | 5 4 5 4 4 4 4 5<br>8 9 9 8 8 9 11 11 | 13896 | 3600.05 | 698 | 300 | 305 | 3664 | 132.59 | 692 | 0 | 1 | 5281 | 41.76 | 893 | 79 | 1059 | 0 |
| (8, 3, 1)(7) | 5 6 6 5 7 4 8 4<br>1 2 3 1 1 4 1 3<br>1 1 1 1 1 1 1 1 | 4 4 4 5 4 4 5 5<br>9 8 9 8 8 11 8 9 | 13768 | 3600.24 | 681 | 253 | 267 | 3664 | 142.19 | 681 | 0 | 2 | 5215 | 41.31 | 914 | 78 | 1077 | 0 |
| (8, 3, 1)(8) | 8 7 5 8 7 8 8 5<br>3 1 4 3 3 4 3 4<br>1 1 1 1 1 1 1 1 | 5 5 5 4 4 5 5 4<br>9 10 11 8 9 10 11 11 | 15560 | 3600.09 | 766 | 322 | 334 | 3664 | 852.59 | 750 | 0 | 3 | 5877 | 44.26 | 972 | 88 | 1192 | 0 |
| (8, 3, 1)(9) | 4 6 7 7 6 5 6 5<br>4 1 1 2 4 1 1 3<br>1 1 1 1 1 1 1 1 | 5 5 4 5 4 5 4 5<br>11 11 8 11 9 11 9 10 | 14536 | 3600.12 | 694 | 283 | 297 | 3664 | 161.34 | 694 | 0 | 2 | 5521 | 43.04 | 907 | 82 | 1119 | 0 |
| (8, 3, 3)(0) | 8 7 7 8 8 5 7 4<br>4 2 4 2 3 4 4 1<br>3 3 3 3 3 3 3 3 | 5 5 5 4 5 5 4 4<br>11 9 11 10 9 9 11 8 | 18056 | 3600.14 | 999 | 450 | 469 | 3664 | 30.51 | 999 | 0 | 2 | 6880 | 80.23 | 1181 | 100 | 1418 | 0 |
| (8, 3, 3)(1) | 7 7 5 5 8 8 6 8<br>3 4 4 2 1 2 1 2<br>3 3 3 3 3 3 3 3 | 5 5 5 5 5 5 5 4<br>8 9 9 9 9 10 9 11 | 17672 | 3600.13 | 1012 | 598 | 635 | 3664 | 28.39 | 1012 | 0 | 1 | 6731 | 79.52 | 1152 | 100 | 1438 | 0 |
| (8, 3, 3)(2) | 8 5 7 6 6 8 4 6<br>4 3 2 2 2 2 1 4<br>3 3 3 3 3 3 3 3 | 4 5 4 4 4 5 5 5<br>11 11 10 10 10 8 11 10 | 17736 | 3600.17 | 1041 | 442 | 442 | 3664 | 25.09 | 1041 | 1 | 2 | 6756 | 79.65 | 1156 | 100 | 1266 | 0 |
| (8, 3, 3)(3) | 5 6 8 6 8 8 5 7<br>2 3 2 2 2 1 4 4<br>3 3 3 3 3 3 3 3 | 5 4 5 5 5 5 5 5<br>10 11 8 9 9 8 10 9 | 17672 | 3600.15 | 1027 | 388 | 388 | 3664 | 28.33 | 1027 | 2 | 2 | 6731 | 79.65 | 1159 | 100 | 1272 | 0 |
| (8, 3, 3)(4) | 8 7 7 8 8 7 5 5<br>2 4 3 2 2 1 1 3<br>3 3 3 3 3 3 3 3 | 5 5 4 5 5 5 5 4<br>9 11 9 11 11 9 8 8 | 17736 | 3600.11 | 990 | 447 | 527 | 3664 | 27.91 | 990 | 0 | 1 | 6753 | 78.73 | 1146 | 100 | 1366 | 0 |
| (8, 3, 3)(5) | 8 6 8 4 8 8 6 4<br>1 3 4 3 1 1 1 1<br>3 3 3 3 3 3 3 3 | 4 4 5 5 5 5 5 5<br>10 9 8 9 11 8 9 8 | 17160 | 3600.23 | 970 | 526 | 526 | 3664 | 26.50 | 969 | 0 | 2 | 6539 | 78.57 | 1120 | 98 | 1294 | 0 |
| (8, 3, 3)(6) | 7 8 8 8 5 4 7 8<br>3 4 3 4 4 4 2 4<br>3 3 3 3 3 3 3 3 | 4 4 4 4 5 4 5 4<br>8 8 8 9 10 8 9 10 | 17736 | 3600.19 | 970 | 605 | 605 | 3664 | 33.41 | 962 | 0 | 1 | 6743 | 80.32 | 1137 | 100 | 1338 | 0 |
| (8, 3, 3)(7) | 5 8 6 7 7 4 4 6<br>3 2 4 3 4 1 4 4<br>3 3 3 3 3 3 3 3 | 5 4 5 5 4 4 4 4<br>8 10 8 8 10 11 10 9 | 17352 | 3600.14 | 978 | 520 | 520 | 3664 | 29.38 | 978 | 0 | 2 | 6622 | 79.62 | 1108 | 99 | 1375 | 0 |
| (8, 3, 3)(8) | 4 7 8 7 8 4 5 4<br>4 1 2 4 3 1 4 4<br>3 3 3 3 3 3 3 3 | 4 4 4 5 5 5 5 5<br>10 9 10 11 10 10 8 8 | 17480 | 3600.09 | 998 | 405 | 471 | 3664 | 27.41 | 998 | 0 | 2 | 6668 | 78.68 | 1132 | 100 | 1357 | 0 |
| (8, 3, 3)(9) | 6 7 8 6 7 5 6 4<br>2 4 2 2 1 4 4 3<br>3 3 3 3 3 3 3 3 | 4 5 5 5 4 4 5 4<br>11 10 8 9 10 10 8 8 | 17352 | 3600.35 | 1004 | 548 | 553 | 3664 | 37.30 | 1004 | 0 | 2 | 6623 | 79.68 | 1086 | 99 | 1375 | 0 |
| (9, 3, 1)(0) | 6 6 7 8 4 4 4 8 8<br>3 1 3 4 4 4 1 3 3<br>1 1 1 1 1 1 1 1 1 | 4 4 4 4 5 4 4 4 5<br>9 8 11 9 10 10 11 11 8 | 18657 | 3600.12 | 963 | 648 | 690 | 4698 | 407.73 | 925 | 0 | 5 | 7139 | 80.68 | 1167 | 100 | 1542 | 0 |
| (9, 3, 1)(1) | 7 6 4 5 5 7 7 8 8<br>4 3 3 4 1 2 3 2 1<br>1 1 1 1 1 1 1 1 1 | 5 5 5 4 5 5 4 5 5<br>9 9 8 11 10 10 10 10 11 | 18945 | 3600.12 | 907 | 560 | 612 | 4698 | 3600.14 | 883 | 3 | 3 | 7265 | 81.22 | 1186 | 100 | 1353 | 0 |
| (9, 3, 1)(2) | 6 4 5 5 4 6 5 5 7<br>1 2 2 2 1 2 3 2 2<br>1 1 1 1 1 1 1 1 1 | 5 4 5 4 4 4 4 4 4<br>10 11 10 11 11 9 8 11 10 | 17793 | 3600.16 | 937 | 530 | 530 | 4698 | 467.83 | 908 | 0 | 2 | 6831 | 78.06 | 1192 | 100 | 1416 | 0 |
| (9, 3, 1)(3) | 6 4 7 5 5 5 6 5 6<br>3 3 2 3 2 2 2 4 2<br>1 1 1 1 1 1 1 1 1 | 4 5 4 4 4 4 5 4 5<br>9 11 8 11 8 11 10 10 9 | 18153 | 3600.19 | 931 | 559 | 601 | 4698 | 986.88 | 899 | 0 | 5 | 6948 | 80.01 | 1120 | 100 | 1445 | 0 |
| (9, 3, 1)(4) | 4 6 6 8 5 7 5 6 7<br>4 4 2 2 3 3 4 2 3<br>1 1 1 1 1 1 1 1 1 | 5 4 4 5 5 5 4 5 4<br>11 11 9 9 8 11 11 11 10 | 19089 | 3600.14 | 916 | 869 | 869 | 4698 | 3600.08 | 900 | 0 | 6 | 7314 | 81.29 | 1166 | 100 | 1491 | 0 |
| (9, 3, 1)(5) | 4 5 4 5 5 7 7 4 8<br>1 2 2 4 1 4 2 4 1<br>1 1 1 1 1 1 1 1 1 | 4 4 4 4 5 5 4 5 4<br>8 8 11 8 9 11 8 9 9 | 17577 | 3600.11 | 884 | 509 | 535 | 4698 | 210.65 | 873 | 0 | 3 | 6750 | 78.46 | 1181 | 100 | 1338 | 0 |
| (9, 3, 1)(6) | 4 6 6 5 6 7 5 4 6<br>3 1 1 1 1 3 1 1 3<br>1 1 1 1 1 1 1 1 1 | 5 4 5 4 4 4 4 5 5<br>9 8 10 11 11 9 8 11 11 | 17721 | 3600.19 | 880 | 873 | 873 | 4698 | 1957.84 | 857 | 0 | 5 | 6806 | 78.55 | 1147 | 100 | 1442 | 0 |
| (9, 3, 1)(7) | 7 4 7 5 7 7 7 5 6<br>4 4 4 3 4 1 4 1 2<br>1 1 1 1 1 1 1 1 1 | 5 4 5 5 5 4 5 5 5<br>8 11 8 9 8 8 11 10 11 | 18801 | 3600.11 | 900 | 690 | 690 | 4698 | 3600.04 | 871 | 0 | 5 | 7213 | 80.31 | 1142 | 100 | 1477 | 0 |
| (9, 3, 1)(8) | 8 6 5 6 4 6 8 7 8<br>2 4 4 3 4 2 3 3 3<br>1 1 1 1 1 1 1 1 1 | 4 5 4 5 4 5 4 5 4<br>11 8 8 10 11 9 8 9 11 | 18945 | 3600.14 | 928 | 900 | 1044 | 4698 | 669.65 | 891 | 0 | 5 | 7259 | 80.46 | 1122 | 100 | 1512 | 0 |
| (9, 3, 1)(9) | 7 8 7 7 5 8 7 4 8<br>3 2 2 4 2 3 3 3 1<br>1 1 1 1 1 1 1 1 1 | 5 4 4 5 5 4 5 5 5<br>11 10 11 11 8 10 9 10 9 | 19233 | 3600.13 | 929 | 1097 | 1097 | 4698 | 3600.07 | 895 | 0 | 9 | 7361 | 81.20 | 1199 | 100 | 1523 | 0 |
| (9, 3, 3)(1) | 8 5 5 4 5 5 4 5 5<br>1 2 2 1 1 3 1 4 3<br>3 3 3 3 3 3 3 3 3 | 4 5 4 4 4 4 4 4 4<br>9 8 10 10 11 9 11 8 9 | 20817 | 3600.15 | 1211 | 623 | 674 | 4698 | 231.25 | 1210 | 0 | 3 | 8042 | 83.83 | 1450 | 100 | 1672 | 0 |

**Supplementary Table S6.** A list with all parameters of the major instance library. The following abbrevations are used: conf-key: The configuration $(N, K, p_3)(nr)$ where $nr \in \{0, \ldots, 9\}$ is the number of the randomly generated instance; process times: the process times of the samples (columns) on sample shaker (row 1), sample mixer (row 2) and photo booth (row 3); gaps: the gaps between subsequent photos of the samples (columns), gap 1 between photo 1 and photo 2 is in row 1 and so on; number of variables (NV); runtime (T); objective value (OV); Sequence model (S); Gurobi with the sequence model (SE-GU); QUBO model (Q);Fujitsu's digital annealer hybrid framework (FDAh) with the QUBO model (QU-FDAh); the relative runtime of SE-GUw.r.t. QU-FDAh (SE-GU@QU-FDAh).

| conf-key | process times | gaps | NV-S | T-SE-GU | OV-SE-GU | SE-GU@QU-FDAh | NV-Q | T-QU-FDAh | OV-QU-FDAh |
|---|---|---|---|---|---|---|---|---|---|
| (8, 4, 3)(1) | 7 8 6 4 8 6 4 6<br>3 1 3 4 3 4 4 3<br>3 3 3 3 3 3 3 3 | 5 5 5 5 4 4 5 5<br>9 8 10 8 8 10 11 9<br>23 19 22 21 20 21 23 16 | 4912 | 25.58 | 1227 | 5 | 11058 | 129 | 1353 |
| (8, 4, 3)(3) | 7 6 6 4 8 7 8 4<br>4 2 2 4 4 4 4 2<br>3 3 3 3 3 3 3 3 | 4 5 5 4 4 4 5 4<br>9 11 9 9 10 9 9 8<br>18 22 16 20 23 16 23 23 | 4912 | 14.65 | 1213 | 5 | 10968 | 128 | 1335 |
| (8, 4, 3)(6) | 6 5 8 6 8 7 7 5<br>4 3 2 1 1 3 2 4<br>3 3 3 3 3 3 3 3 | 5 5 4 5 4 5 5 4<br>10 10 8 8 8 8 11 9<br>20 22 16 22 21 22 19 22 | 4912 | 20.31 | 1236 | 5 | 10950 | 129 | 1392 |
| (8, 4, 3)(7) | 4 4 4 5 6 8 7 6<br>4 3 4 3 4 2 2 2<br>3 3 3 3 3 3 3 3 | 5 5 5 4 5 5 4 5<br>10 10 8 8 9 9 9 11<br>22 22 19 21 21 18 17 19 | 4912 | 23.80 | 1216 | 9 | 10822 | 127 | 1279 |
| (9, 4, 1)(0) | 8 7 6 8 5 7 6 7 4<br>3 3 4 3 1 2 2 3 3<br>1 1 1 1 1 1 1 1 1 | 4 4 4 4 5 5 4 4 4<br>10 8 8 11 10 8 11 10 10<br>19 21 19 23 21 18 23 19 21 | 6300 | 332.80 | 1224 | 18 | 12206 | 144 | 1362 |
| (9, 4, 1)(1) | 6 7 4 4 5 7 8 7 5<br>1 4 4 2 3 2 4 1 2<br>1 1 1 1 1 1 1 1 1 | 5 5 4 5 5 4 5 4 4<br>10 11 9 9 9 11 10 8 8<br>18 18 17 16 23 20 19 19 20 | 6300 | 591.54 | 1155 | 3 | 11762 | 137 | 1397 |
| (9, 4, 1)(2) | 7 8 6 8 8 6 4 6 5<br>4 3 4 3 1 2 3 4 2<br>1 1 1 1 1 1 1 1 1 | 4 4 5 5 4 5 5 4 5<br>11 10 10 9 9 8 9 9 9<br>20 18 16 23 21 21 21 21 17 | 6300 | 1387.17 | 1183 | 16 | 12129 | 142 | 1388 |
| (9, 4, 1)(3) | 7 6 6 7 4 7 4 4 6<br>4 4 4 4 4 1 3 1 1<br>1 1 1 1 1 1 1 1 1 | 5 5 4 5 5 5 5 4 4<br>9 9 8 10 8 11 8 10 9<br>23 20 20 16 23 19 21 18 22 | 6300 | 688.51 | 1183 | 7 | 12036 | 141 | 1426 |
| (9, 4, 1)(4) | 5 4 5 7 8 4 4 8 6<br>3 3 2 2 3 3 4 3 1<br>1 1 1 1 1 1 1 1 1 | 5 4 5 5 5 5 4 5 4<br>8 11 8 9 11 10 9 11 11<br>16 21 16 19 19 19 22 23 21 | 6300 | 1306.01 | 1150 | 21 | 11988 | 139 | 1301 |
| (9, 4, 1)(5) | 7 5 7 5 5 7 4 5 4<br>2 2 3 4 4 1 3 4 1<br>1 1 1 1 1 1 1 1 1 | 4 4 5 5 4 5 4 5 5<br>9 11 9 8 9 8 10 8 10<br>17 20 18 22 18 23 18 16 17 | 6300 | 808.45 | 1142 | 31 | 11590 | 136 | 1290 |
| (9, 4, 1)(6) | 6 6 7 7 5 8 5 5 5<br>4 2 2 3 4 4 1 2 2<br>1 1 1 1 1 1 1 1 1 | 4 5 4 5 4 4 5 4 5<br>8 8 10 11 11 11 9 11 9<br>23 23 17 16 17 21 19 20 19 | 6300 | 729.75 | 1171 | 31 | 11985 | 140 | 1291 |
| (9, 4, 1)(7) | 4 8 6 8 6 8 5 5 4<br>3 2 1 2 4 4 3 4 3<br>1 1 1 1 1 1 1 1 1 | 4 5 5 5 5 5 5 4 4<br>11 10 9 8 11 8 10 8 10<br>21 23 22 18 21 21 22 16 19 | 6300 | 843.09 | 1166 | 9 | 12208 | 144 | 1379 |
| (9, 4, 1)(8) | 5 6 7 5 4 8 8 4 5<br>2 4 3 2 2 1 3 4 1<br>1 1 1 1 1 1 1 1 1 | 5 5 4 5 5 4 4 4 4<br>11 11 8 11 9 8 8 10 9<br>16 22 22 22 23 18 21 19 22 | 6300 | 924.76 | 1185 | 29 | 12064 | 142 | 1341 |
| (9, 4, 1)(9) | 7 7 4 4 8 7 8 4 5<br>2 4 2 2 4 2 2 2 3<br>1 1 1 1 1 1 1 1 1 | 4 5 4 5 5 4 5 5 5<br>10 9 11 11 10 11 10 10 10<br>23 23 20 18 23 23 17 22 18 | 6300 | 2291.52 | 1200 | 5 | 12411 | 144 | 1435 |
| (9, 4, 3)(0) | 4 5 5 5 5 4 6 6 8<br>2 1 4 4 2 3 4 4 2<br>3 3 3 3 3 3 3 3 3 | 4 4 4 4 5 4 5 4 4<br>9 9 11 9 9 9 10 9 8<br>21 19 16 23 22 21 18 18 23 | 6300 | 126.14 | 1479 | 16 | 13700 | 160 | 1523 |
| (9, 4, 3)(1) | 8 6 5 8 6 5 4 4 4<br>3 2 2 4 3 2 2 4 4<br>3 3 3 3 3 3 3 3 3 | 5 4 5 5 4 4 4 5 5<br>10 9 9 11 8 9 10 8 9<br>16 21 21 21 18 23 20 17 17 | 6300 | 156.16 | 1466 | 3 | 13648 | 160 | 1772 |
| (9, 4, 3)(2) | 8 5 7 4 5 8 5 8 5<br>2 2 3 3 1 2 3 1 3<br>3 3 3 3 3 3 3 3 3 | 4 5 5 5 5 5 4 4 5<br>8 10 10 10 11 9 9 8 9<br>21 19 23 21 20 23 17 18 16 | 6300 | 160.52 | 1468 | 3 | 13774 | 162 | 1603 |
| (9, 4, 3)(3) | 4 7 4 8 4 5 4 6 5<br>2 1 2 1 1 4 1 3 3<br>3 3 3 3 3 3 3 3 3 | 4 5 5 4 5 5 4 4 5<br>10 11 10 11 10 11 11 8 10<br>19 16 19 23 18 17 23 17 18 | 6300 | 210.02 | 1477 | 12 | 13509 | 158 | 1568 |
| (9, 4, 3)(4) | 7 6 8 6 8 8 7 6 7<br>4 3 4 4 2 4 3 2 4<br>3 3 3 3 3 3 3 3 3 | 4 4 5 5 5 5 4 5 5<br>8 8 10 8 11 9 8 10 10<br>19 23 21 17 16 19 19 19 23 | 6300 | 164.56 | 1490 | 3 | 14106 | 166 | 1712 |
| (9, 4, 3)(5) | 6 8 6 8 6 4 5 6 6<br>2 3 1 1 2 4 1 1 4<br>3 3 3 3 3 3 3 3 3 | 5 5 5 4 4 4 4 4 4<br>9 10 8 8 10 9 9 9 9<br>22 20 17 20 17 16 23 16 16 | 6300 | 99.81 | 1432 | 3 | 13325 | 157 | 1804 |
| (9, 4, 3)(6) | 8 7 4 5 5 4 8 5 4<br>1 1 3 3 1 3 3 2 2<br>3 3 3 3 3 3 3 3 3 | 5 4 5 4 5 5 5 5 5<br>9 8 11 11 8 11 10 8 10<br>23 17 16 16 20 22 17 16 18 | 6300 | 79.35 | 1444 | 3 | 13380 | 157 | 1719 |
| (9, 4, 3)(7) | 8 5 7 8 4 6 4 6 7<br>1 2 4 2 1 4 3 3 1<br>3 3 3 3 3 3 3 3 3 | 4 4 4 4 4 5 5 4 5<br>11 9 8 10 11 10 10 9 10<br>19 23 19 23 22 23 22 21 16 | 6300 | 182.01 | 1520 | 3 | 14073 | 164 | 1655 |
| (9, 4, 3)(8) | 4 8 8 4 4 7 4 4 4<br>1 1 3 2 1 3 3 2 4<br>3 3 3 3 3 3 3 3 3 | 4 5 4 5 5 5 5 4 4<br>10 9 9 9 9 10 11 9 9<br>21 22 16 20 18 16 17 18 20 | 6300 | 187.09 | 1436 | 20 | 13332 | 156 | 1611 |
| (9, 4, 3)(9) | 5 6 8 7 5 4 6 7 7<br>2 2 3 2 3 3 1 3 4<br>3 3 3 3 3 3 3 3 3 | 4 5 5 5 4 5 4 5 5<br>11 10 10 10 8 9 9 11 8<br>19 23 16 17 21 22 22 22 19 | 6300 | 180.34 | 1490 | 20 | 13971 | 162 | 1573 |
| (10, 3, 3)(0) | 8 7 8 8 7 7 6 7 5 6<br>2 4 3 3 4 3 1 4 1 2<br>3 3 3 3 3 3 3 3 3 3 | 4 5 5 5 5 5 4 5 4 5<br>8 10 11 10 11 8 10 11 11 11 | 5860 | 1498.77 | 1541 | 16 | 11026 | 129 | 1605 |
| (10, 4, 1)(0) | 4 7 4 8 7 4 7 4 6 6<br>3 3 3 3 2 2 4 3 2 3<br>1 1 1 1 1 1 1 1 1 1 | 5 4 4 4 5 4 4 5 5 5<br>11 8 10 8 9 11 9 8 11 8<br>23 19 18 22 19 19 19 20 21 18 | 7860 | 3600.01 | 1444 | 55 | 14853 | 174 | 1653 |
| (10, 4, 1)(1) | 6 7 8 5 5 4 7 7 6 4<br>4 2 1 3 1 3 3 2 1 4<br>1 1 1 1 1 1 1 1 1 1 | 5 4 4 5 5 4 4 4 4 4<br>10 11 10 9 9 10 11 8 11 8<br>20 23 18 20 16 23 23 20 18 20 | 7860 | 3600.02 | 1430 | 38 | 14939 | 174 | 1665 |
| (10, 4, 1)(2) | 5 7 6 8 8 5 8 4 6 8<br>2 4 1 1 1 4 1 1 2 1<br>1 1 1 1 1 1 1 1 1 1 | 5 4 5 4 5 4 4 5 4 4<br>10 11 9 9 11 9 10 8 8 11<br>16 16 19 16 22 20 19 23 19 16 | 7860 | 3600.01 | 1352 | 51 | 14519 | 170 | 1554 |
| (10, 4, 1)(3) | 5 7 6 8 4 7 7 4 8 7<br>2 2 2 3 4 2 2 4 2 1<br>1 1 1 1 1 1 1 1 1 1 | 5 5 4 5 4 5 5 4 5 4<br>9 10 8 10 9 11 11 11 11 11<br>22 21 16 18 17 18 19 23 16 20 | 7860 | 3600.01 | 1418 | 62 | 14935 | 175 | 1629 |
| (10, 4, 1)(4) | 6 4 4 7 7 7 7 6 6 8<br>3 1 4 4 1 1 3 4 2 1<br>1 1 1 1 1 1 1 1 1 1 | 5 4 5 4 4 4 4 5 5 4<br>11 9 9 10 9 11 10 8 11 9<br>19 20 18 17 17 17 19 16 22 23 | 7860 | 3281.14 | 1428 | 32 | 14684 | 171 | 1579 |
| (10, 4, 1)(5) | 5 7 8 7 7 4 7 5 8 6<br>2 4 4 4 2 3 3 2 2 2<br>1 1 1 1 1 1 1 1 1 1 | 4 5 4 5 5 4 5 5 5 5<br>8 11 11 9 9 8 9 9 11 10<br>20 21 17 23 16 18 22 17 23 21 | 7860 | 3600.01 | 1411 | 30 | 15154 | 176 | 1606 |
| (10, 4, 1)(6) | 7 6 6 4 5 6 6 6 6 4<br>2 2 3 4 4 1 3 1 3 3<br>1 1 1 1 1 1 1 1 1 1 | 5 5 4 5 5 4 4 5 4 5<br>9 9 8 9 11 8 11 11 10 11<br>23 21 19 23 16 16 23 20 22 19 | 7860 | 3600.01 | 1449 | 58 | 15024 | 175 | 1587 |
| (10, 4, 1)(7) | 8 5 4 4 7 8 7 6 5 4<br>4 1 3 2 4 3 2 4 1 2<br>1 1 1 1 1 1 1 1 1 1 | 5 5 4 4 4 4 5 4 5 5<br>11 11 10 10 11 9 9 8 11 11<br>19 21 19 20 23 17 23 18 22 21 | 7860 | 3600.01 | 1400 | 11 | 15190 | 176 | 1770 |
| (10, 4, 1)(8) | 6 4 4 4 4 4 7 6 7 6<br>4 1 2 2 2 1 1 2 3 1<br>1 1 1 1 1 1 1 1 1 1 | 4 4 4 5 5 5 4 4 5 4<br>9 11 8 11 8 8 8 9 9 9<br>18 23 23 16 23 19 22 17 18 17 | 7860 | 3600.02 | 1438 | 58 | 14307 | 167 | 1578 |
| (10, 4, 1)(9) | 7 7 6 4 6 6 8 5 5 6<br>1 2 2 2 2 4 3 2 3 3<br>1 1 1 1 1 1 1 1 1 1 | 5 4 5 5 4 4 5 5 4 5<br>10 9 8 11 11 9 11 8 10 9<br>21 17 20 17 20 19 22 22 16 21 | 7860 | 3600.01 | 1402 | 88 | 14854 | 174 | 1545 |
| (10, 4, 3)(0) | 7 4 4 7 8 7 7 7 5 4<br>3 4 1 1 2 4 1 3 4 2<br>3 3 3 3 3 3 3 3 3 3 | 4 5 5 4 4 4 5 4 4 4<br>11 9 11 11 9 9 9 9 10 10<br>20 16 21 23 17 23 21 20 18 19 | 7860 | 1575.98 | 1772 | 36 | 17217 | 200 | 1872 |
| (10, 4, 3)(1) | 5 8 6 6 7 4 6 5 5 7<br>1 4 4 1 1 1 3 1 3 3<br>3 3 3 3 3 3 3 3 3 3 | 5 4 4 5 4 4 4 4 4 4<br>11 9 9 8 10 11 9 10 9 11<br>21 17 18 23 23 20 19 17 16 18 | 7860 | 1382.11 | 1725 | 25 | 16885 | 197 | 1975 |
| (10, 4, 3)(2) | 8 5 5 8 7 8 6 4 8 4<br>3 2 1 2 2 2 3 1 3 1<br>3 3 3 3 3 3 3 3 3 3 | 5 4 5 4 4 5 4 5 4 5<br>9 8 9 11 9 11 10 9 10 11<br>22 19 23 16 22 22 22 18 23 19 | 7860 | 1297.17 | 1802 | 5 | 17415 | 202 | 1950 |
| (10, 4, 3)(3) | 7 4 5 6 6 4 7 7 4 8<br>3 1 3 3 4 2 1 1 4 3<br>3 3 3 3 3 3 3 3 3 3 | 4 5 5 5 5 4 5 5 4 4<br>11 9 11 10 8 8 10 10 9 9<br>19 21 19 18 17 23 19 16 22 23 | 7860 | 1484.50 | 1773 | 5 | 17135 | 201 | 1882 |
| (10, 4, 3)(4) | 7 5 7 6 4 8 5 8 8 7<br>1 3 4 4 3 1 4 1 2 4<br>3 3 3 3 3 3 3 3 3 3 | 5 4 4 4 5 4 5 5 5 4<br>10 8 10 10 9 9 10 10 9 9<br>17 20 22 17 22 23 16 18 18 16 | 7860 | 1674.06 | 1770 | 15 | 17098 | 199 | 1993 |
| (10, 4, 3)(5) | 7 6 7 7 7 8 7 4 6 7<br>1 3 2 3 1 1 3 1 3 2<br>3 3 3 3 3 3 3 3 3 3 | 4 5 4 5 5 4 5 4 5 5<br>8 9 9 11 10 10 8 10 9 11<br>23 21 22 22 22 22 22 18 20 18 | 7860 | 2003.74 | 1819 | 24 | 17580 | 204 | 1942 |
| (10, 4, 3)(6) | 6 7 4 6 7 6 8 6 7 8<br>3 4 4 3 2 1 2 1 4 1<br>3 3 3 3 3 3 3 3 3 3 | 4 4 5 5 4 4 4 5 4 5<br>10 10 11 10 11 9 11 8 11 9<br>16 17 17 16 17 23 23 20 16 21 | 7860 | 914.92 | 1767 | 4 | 17100 | 201 | 2045 |
| (10, 4, 3)(7) | 7 4 8 5 6 8 6 5 7 7<br>2 1 3 2 4 4 4 4 4 2<br>3 3 3 3 3 3 3 3 3 3 | 4 5 5 5 5 5 4 4 5 4<br>11 8 9 11 9 10 9 8 11 11<br>16 21 19 16 16 17 19 16 18 21 | 7860 | 688.70 | 1731 | 11 | 16957 | 197 | 2108 |
| (10, 4, 3)(8) | 4 6 8 4 7 6 4 5 4 5<br>2 1 2 3 4 4 2 2 1 1<br>3 3 3 3 3 3 3 3 3 3 | 5 5 5 5 5 4 4 5 5 5<br>9 8 11 8 9 9 9 11 9 10<br>19 23 19 23 19 23 17 19 17 16 | 7860 | 821.36 | 1774 | 35 | 16863 | 196 | 1858 |
| (10, 4, 3)(9) | 5 6 4 5 8 4 4 7 6 5<br>1 2 1 4 1 4 3 3 1 1<br>3 3 3 3 3 3 3 3 3 3 | 5 5 4 4 5 4 4 4 5 5<br>9 11 9 10 8 11 10 9 8 9<br>22 18 19 21 19 20 17 21 22 17 | 7860 | 1416.27 | 1747 | 15 | 16835 | 198 | 1938 |
| (15, 2, 1)(0) | 7 6 6 8 6 7 5 8 4 6 6 8 5 5 8<br>4 1 2 1 4 3 4 4 1 3 4 1 3 2 2<br>1 1 1 1 1 1 1 1 1 1 1 1 1 1 1 | 5 5 5 4 5 5 5 4 4 4 4 5 4 5 5 | 9360 | 3600.16 | 1644 | 68 | 13155 | 153 | 1707 |
| (15, 2, 1)(1) | 4 5 5 5 4 5 8 5 5 7 5 4 7 6 7<br>4 4 4 3 4 4 4 2 2 1 3 3 1 1 1<br>1 1 1 1 1 1 1 1 1 1 1 1 1 1 1 | 4 4 4 4 4 4 5 5 4 5 5 4 4 5 4 | 9360 | 3600.02 | 1569 | 462 | 12521 | 146 | 1662 |
| (15, 2, 1)(2) | 7 8 5 8 4 7 8 5 6 7 7 6 6 4 8<br>3 1 1 2 1 4 1 4 2 1 2 2 4 4 2<br>1 1 1 1 1 1 1 1 1 1 1 1 1 1 1 | 5 5 5 5 4 5 5 5 5 5 4 5 5 4 5 | 9360 | 3600.03 | 1641 | 69 | 13116 | 154 | 1780 |
| (15, 2, 1)(3) | 7 6 4 6 4 6 6 4 7 7 6 4 4 8 6<br>2 2 1 3 4 3 3 2 4 2 2 3 2 1 4<br>1 1 1 1 1 1 1 1 1 1 1 1 1 1 1 | 4 4 5 5 5 5 5 5 5 5 4 5 5 5 4 | 9360 | 3600.07 | 1701 | 145 | 12779 | 149 | 1755 |
| (15, 2, 1)(4) | 4 4 6 6 6 7 5 8 6 6 6 5 5 8 5<br>2 2 1 1 2 1 3 2 3 3 2 2 2 1 2<br>1 1 1 1 1 1 1 1 1 1 1 1 1 1 1 | 4 4 4 4 4 4 5 4 5 5 4 5 4 5 5 | 9360 | 3600.01 | 1557 | 1013 | 12270 | 144 | 1597 |
| (15, 2, 1)(5) | 7 6 7 6 6 8 6 7 4 7 6 8 4 8 6<br>2 1 2 1 2 4 3 3 1 3 2 4 2 3 2<br>1 1 1 1 1 1 1 1 1 1 1 1 1 1 1 | 5 4 5 4 5 4 4 5 4 4 4 5 5 5 5 | 9360 | 3600.40 | 1642 | 128 | 12986 | 153 | 1687 |
| (15, 2, 1)(6) | 8 6 6 8 5 7 8 5 5 8 5 5 5 4 5<br>1 1 2 4 4 3 4 4 1 4 4 4 2 3 3<br>1 1 1 1 1 1 1 1 1 1 1 1 1 1 1 | 4 4 5 5 5 5 4 5 4 4 4 4 5 4 4 | 9360 | 3600.03 | 1616 | 355 | 13026 | 152 | 1648 |
| (15, 2, 1)(7) | 7 8 6 7 4 8 5 5 4 5 6 7 8 8 4<br>1 4 1 3 1 4 4 3 2 4 4 3 3 1 1<br>1 1 1 1 1 1 1 1 1 1 1 1 1 1 1 | 5 5 5 4 5 4 4 5 4 5 4 4 4 5 5 | 9360 | 3600.03 | 1643 | 66 | 13029 | 151 | 1703 |
| (15, 2, 1)(8) | 5 4 4 5 5 4 7 7 5 4 4 5 5 4 6<br>4 4 4 2 3 4 3 3 3 3 3 1 3 1 1<br>1 1 1 1 1 1 1 1 1 1 1 1 1 1 1 | 4 5 4 4 4 4 5 5 5 5 5 5 4 4 5 | 9360 | 3600.10 | 1602 | 82 | 12356 | 144 | 1650 |
| (15, 2, 1)(9) | 6 4 6 7 8 5 6 7 5 5 5 7 4 7 6<br>1 2 3 3 4 1 3 2 1 3 1 1 2 3 3<br>1 1 1 1 1 1 1 1 1 1 1 1 1 1 1 | 4 5 4 4 5 4 5 5 4 5 5 4 4 4 5 | 9360 | 3600.07 | 1536 | 78 | 12523 | 146 | 1665 |
| (15, 2, 3)(0) | 8 8 8 4 6 6 4 6 6 7 8 6 8 8 4<br>1 3 3 3 4 4 3 2 2 4 4 3 4 3 4<br>3 3 3 3 3 3 3 3 3 3 3 3 3 3 3 | 5 5 4 4 4 5 5 5 5 4 4 4 4 5 4 | 9360 | 3600.11 | 1855 | 131 | 16129 | 188 | 1929 |
| (15, 2, 3)(1) | 4 6 5 6 7 7 5 8 6 8 7 7 7 8 7<br>4 1 1 3 4 4 4 2 1 2 4 3 1 4 2<br>3 3 3 3 3 3 3 3 3 3 3 3 3 3 3 | 5 5 4 5 5 4 4 4 4 5 4 5 5 5 4 | 9360 | 3600.19 | 1880 | 93 | 15920 | 185 | 2043 |
| (15, 2, 3)(2) | 7 4 6 7 6 4 5 8 8 4 4 7 8 8 6<br>1 1 1 4 1 4 1 3 2 4 3 3 1 2 1<br>3 3 3 3 3 3 3 3 3 3 3 3 3 3 3 | 5 5 5 4 4 4 4 5 5 5 5 4 5 4 4 | 9360 | 3600.07 | 1835 | 194 | 15332 | 178 | 1936 |
| (15, 2, 3)(3) | 5 6 5 4 6 7 6 8 5 5 7 6 8 7 6<br>2 4 2 3 3 1 3 4 1 4 4 2 1 2 3<br>3 3 3 3 3 3 3 3 3 3 3 3 3 3 3 | 4 4 4 5 5 5 4 4 5 4 4 4 4 4 5 | 9360 | 3600.04 | 1840 | 55 | 15455 | 181 | 2001 |
| (15, 2, 3)(4) | 8 4 7 6 7 7 6 8 6 5 5 6 8 4 8<br>1 1 2 3 3 2 3 3 2 4 4 3 1 3 3<br>3 3 3 3 3 3 3 3 3 3 3 3 3 3 3 | 5 4 5 5 4 5 4 4 5 5 5 4 4 4 5 | 9360 | 3600.11 | 1847 | 120 | 15710 | 183 | 1997 |
| (15, 2, 3)(5) | 7 4 8 8 7 8 7 6 7 4 4 6 6 5 7<br>3 2 2 3 1 1 4 4 2 1 1 1 2 2 2<br>3 3 3 3 3 3 3 3 3 3 3 3 3 3 3 | 4 4 4 4 5 4 5 5 5 4 4 4 5 5 4 | 9360 | 3600.05 | 1896 | 44 | 15331 | 180 | 2042 |
| (15, 2, 3)(6) | 6 5 7 5 6 5 4 4 8 4 5 8 7 4 5<br>3 1 1 2 4 4 4 1 4 2 2 4 3 3 2<br>3 3 3 3 3 3 3 3 3 3 3 3 3 3 3 | 4 4 4 5 5 4 4 5 5 4 4 4 4 4 5 | 9360 | 3600.24 | 1892 | 40 | 15204 | 177 | 1986 |
| (15, 2, 3)(7) | 4 6 6 5 8 7 8 7 8 8 6 4 6 4 4<br>3 4 3 4 3 1 1 2 3 3 2 3 4 4 4<br>3 3 3 3 3 3 3 3 3 3 3 3 3 3 3 | 4 5 4 5 5 4 5 5 4 4 4 5 5 4 4 | 9360 | 3600.04 | 1832 | 261 | 15751 | 183 | 1977 |
| (15, 2, 3)(8) | 7 6 7 7 7 4 8 7 8 8 5 6 8 4 6<br>1 3 3 2 1 1 1 2 3 1 4 1 2 3 3<br>3 3 3 3 3 3 3 3 3 3 3 3 3 3 3 | 5 5 4 4 4 4 5 5 5 5 5 4 4 4 5 | 9360 | 3600.02 | 1872 | 41 | 15542 | 181 | 2011 |
| (15, 2, 3)(9) | 4 4 8 4 6 5 7 5 7 8 5 6 8 5 6<br>4 2 3 2 2 1 2 4 1 1 2 3 2 4 4<br>3 3 3 3 3 3 3 3 3 3 3 3 3 3 3 | 4 4 5 5 5 4 4 5 5 5 4 5 4 4 4 | 9360 | 3600.05 | 1907 | 139 | 15331 | 179 | 2031 |
| (15, 3, 1)(0) | 6 5 4 6 6 7 8 5 7 7 6 5 6 7 5<br>1 4 2 4 3 3 2 2 2 1 4 3 3 4 4<br>1 1 1 1 1 1 1 1 1 1 1 1 1 1 1 | 5 4 4 4 5 5 5 5 5 4 5 4 4 5 5<br>9 11 9 9 9 9 9 10 10 11 8 10 10 9 10 | 13590 | 3600.17 | 2266 | 63 | 20540 | 238 | 2713 |
| (15, 3, 1)(1) | 5 5 7 6 5 6 8 7 4 7 6 5 7 4 8<br>1 3 4 3 3 4 2 4 3 2 3 1 1 3 4<br>1 1 1 1 1 1 1 1 1 1 1 1 1 1 1 | 4 5 4 5 4 5 4 4 4 4 4 4 4 5 5<br>10 9 9 8 9 11 11 9 11 11 9 11 8 10 8 | 13590 | 3600.16 | 2329 | 67 | 20412 | 239 | 2610 |
| (15, 3, 1)(2) | 7 5 4 7 5 8 5 4 8 5 7 8 5 4 5<br>4 4 3 1 1 1 3 2 1 2 1 3 2 4 4<br>1 1 1 1 1 1 1 1 1 1 1 1 1 1 1 | 5 4 4 5 5 4 4 4 4 5 5 4 4 4 5<br>10 11 11 11 11 8 9 10 11 11 8 9 10 10 8 | 13590 | 3600.04 | 2274 | 55 | 20248 | 235 | 2671 |
| (15, 3, 1)(3) | 6 8 5 7 7 7 4 8 6 5 5 8 4 4 4<br>2 1 1 4 2 1 2 1 2 4 3 2 2 1 3<br>1 1 1 1 1 1 1 1 1 1 1 1 1 1 1 | 4 5 5 4 4 4 5 5 4 4 5 5 4 5 5<br>10 10 10 9 9 11 9 9 9 11 10 9 8 9 11 | 13590 | 3600.17 | 2346 | 214 | 19994 | 233 | 2423 |
| (15, 3, 1)(4) | 8 6 4 7 6 7 6 5 5 7 7 8 4 6 6<br>3 2 2 2 4 4 3 4 2 2 1 4 4 2 3<br>1 1 1 1 1 1 1 1 1 1 1 1 1 1 1 | 4 5 5 5 5 4 4 4 5 4 4 5 4 5 5<br>8 10 8 8 11 11 10 10 8 9 11 8 11 9 11 | 13590 | 3600.02 | 2356 | 132 | 20581 | 240 | 2537 |
| (15, 3, 1)(5) | 8 6 5 7 4 5 8 4 7 5 4 7 6 5 4<br>4 2 4 2 3 1 2 4 1 3 4 4 2 4 1<br>1 1 1 1 1 1 1 1 1 1 1 1 1 1 1 | 4 4 4 5 4 5 4 5 5 5 4 5 5 5 5<br>8 8 11 9 11 8 8 10 8 9 11 10 8 8 10 | 13590 | 3600.05 | 2238 | 170 | 20030 | 233 | 2424 |
| (15, 3, 1)(6) | 5 7 8 7 6 4 6 4 8 4 8 8 5 5 7<br>1 4 4 3 3 3 3 2 3 3 3 4 4 4 3<br>1 1 1 1 1 1 1 1 1 1 1 1 1 1 1 | 4 4 4 4 5 4 4 4 4 5 5 4 4 5 4<br>9 8 8 9 8 11 9 10 8 8 9 10 8 8 9 | 13590 | 3600.29 | 2319 | 67 | 20146 | 235 | 2723 |
| (15, 3, 1)(7) | 7 5 4 7 7 7 4 8 8 4 4 6 7 4 8<br>1 2 1 3 4 1 1 1 1 4 2 1 3 4 4<br>1 1 1 1 1 1 1 1 1 1 1 1 1 1 1 | 5 4 4 4 5 4 4 5 5 4 5 5 5 4 5<br>9 8 8 9 10 8 9 9 9 11 11 9 9 8 8 | 13590 | 3600.02 | 2280 | 128 | 19775 | 230 | 2503 |
| (15, 3, 1)(8) | 6 5 7 6 4 5 6 7 6 6 7 8 6 4 5<br>2 3 2 2 2 4 1 3 3 4 4 4 1 2 3<br>1 1 1 1 1 1 1 1 1 1 1 1 1 1 1 | 5 5 4 5 5 4 5 4 4 5 4 4 4 5 4<br>9 8 11 8 11 9 9 8 10 8 10 10 9 9 8 | 13590 | 3600.21 | 2323 | 203 | 20028 | 235 | 2414 |
| (15, 3, 1)(9) | 6 5 5 7 8 5 6 4 5 8 4 7 6 4 5<br>3 4 3 2 1 3 1 3 2 1 4 2 4 4 3<br>1 1 1 1 1 1 1 1 1 1 1 1 1 1 1 | 5 4 5 5 4 4 4 4 5 4 4 4 5 4 5<br>10 8 9 9 8 9 10 11 8 11 9 10 11 8 9 | 13590 | 3600.03 | 2259 | 164 | 19988 | 233 | 2494 |
| (20, 1, 1)(0) | 7 4 8 5 7 4 5 8 8 4 7 5 6 6 6 5 4 8 6 7<br>3 4 3 3 4 2 3 2 2 1 3 4 3 1 2 2 1 4 1 1<br>1 1 1 1 1 1 1 1 1 1 1 1 1 1 1 1 1 1 1 1 | | 10000 | 3600.06 | 1982 | 3600 | 15453 | 182 | 1993 |
| (20, 1, 1)(1) | 7 8 7 5 6 5 4 7 5 7 5 5 4 5 4 7 5 8 7 5<br>1 1 3 4 1 4 1 1 4 2 4 4 4 2 1 2 4 2 1 2<br>1 1 1 1 1 1 1 1 1 1 1 1 1 1 1 1 1 1 1 1 | | 10000 | 3600.03 | 2160 | 3600 | 15168 | 177 | 2028 |
| (20, 1, 1)(2) | 5 7 8 5 5 8 4 8 6 7 7 4 5 7 4 7 7 6 4 5<br>2 4 4 2 4 1 3 3 2 3 4 3 1 1 3 4 4 4 2 3<br>1 1 1 1 1 1 1 1 1 1 1 1 1 1 1 1 1 1 1 1 | | 10000 | 3600.06 | 2007 | 2060 | 15852 | 186 | 2039 |
| (20, 1, 1)(3) | 5 6 7 8 6 4 5 4 4 5 8 5 6 6 4 8 5 6 5 5<br>3 4 2 4 1 1 4 1 2 3 3 1 2 2 2 2 2 3 2 4<br>1 1 1 1 1 1 1 1 1 1 1 1 1 1 1 1 1 1 1 1 | | 10000 | 3600.02 | 2032 | 618 | 14940 | 175 | 2068 |
| (20, 1, 1)(4) | 5 5 6 8 5 7 7 7 6 8 6 4 4 7 8 8 7 8 8 7<br>4 1 1 2 2 2 1 1 3 4 3 3 3 4 3 3 4 2 3 2<br>1 1 1 1 1 1 1 1 1 1 1 1 1 1 1 1 1 1 1 1 | | 10000 | 3600.03 | 1974 | 237 | 16194 | 188 | 2095 |
| (20, 1, 1)(5) | 6 4 5 7 6 8 5 7 4 5 5 6 8 4 6 8 5 4 8 6<br>2 3 4 4 4 1 1 2 2 2 2 2 2 4 4 4 3 1 2 4<br>1 1 1 1 1 1 1 1 1 1 1 1 1 1 1 1 1 1 1 1 | | 10000 | 3600.09 | 2094 | 3600 | 15510 | 182 | 1987 |
| (20, 1, 1)(6) | 7 6 6 7 5 7 6 6 4 7 5 5 6 6 6 8 8 5 6 4<br>3 3 1 4 3 4 1 3 1 3 1 3 4 1 4 1 3 1 1 1<br>1 1 1 1 1 1 1 1 1 1 1 1 1 1 1 1 1 1 1 1 | | 10000 | 3600.03 | 1932 | 106 | 15282 | 178 | 2098 |
| (20, 1, 1)(7) | 6 4 6 7 5 6 8 6 5 7 7 8 7 4 4 8 6 4 5 6<br>2 1 2 1 3 3 1 3 4 1 2 1 1 4 4 1 3 3 1 4<br>1 1 1 1 1 1 1 1 1 1 1 1 1 1 1 1 1 1 1 1 | | 10000 | 3600.30 | 2165 | 3600 | 15168 | 177 | 2062 |
| (20, 1, 1)(8) | 6 6 7 5 5 7 6 4 6 7 6 6 5 6 4 5 4 6 4 8<br>1 3 1 3 1 1 3 2 1 3 1 1 4 1 4 4 3 1 2 4<br>1 1 1 1 1 1 1 1 1 1 1 1 1 1 1 1 1 1 1 1 | | 10000 | 3600.02 | 2164 | 3600 | 14769 | 173 | 2002 |
| (20, 1, 1)(9) | 6 7 4 4 5 4 4 8 6 7 6 4 5 6 4 4 4 8 4 7<br>1 3 3 3 3 2 2 1 2 1 2 3 1 2 4 2 2 3 2 4<br>1 1 1 1 1 1 1 1 1 1 1 1 1 1 1 1 1 1 1 1 | | 10000 | 3600.07 | 2041 | 2012 | 14541 | 170 | 2099 |
| (20, 1, 3)(0) | 5 8 5 7 6 6 4 4 5 8 8 7 6 7 4 7 6 6 5 6<br>1 1 3 1 4 1 3 3 1 2 2 2 2 3 3 3 3 4 4 4<br>3 3 3 3 3 3 3 3 3 3 3 3 3 3 3 3 3 3 3 3 | | 10000 | 3600.03 | 2113 | 266 | 17910 | 210 | 2292 |
| (20, 1, 3)(1) | 4 4 8 4 6 7 5 6 6 4 8 5 8 5 6 8 5 6 5 7<br>1 3 3 4 4 2 3 2 2 2 4 3 1 2 2 4 3 3 1 4<br>3 3 3 3 3 3 3 3 3 3 3 3 3 3 3 3 3 3 3 3 | | 10000 | 3600.05 | 2159 | 2439 | 17910 | 210 | 2284 |
| (20, 1, 3)(2) | 4 8 8 4 8 4 8 7 6 8 8 6 4 4 6 5 6 6 4 6<br>1 1 4 1 3 2 4 4 4 1 2 2 3 2 1 1 1 1 2 1<br>3 3 3 3 3 3 3 3 3 3 3 3 3 3 3 3 3 3 3 3 | | 10000 | 3600.03 | 2154 | 95 | 17397 | 204 | 2254 |
| (20, 1, 3)(3) | 5 8 4 6 7 8 4 5 5 6 7 8 8 4 6 4 6 4 5 6<br>3 2 1 4 3 3 3 4 3 3 3 2 2 1 3 1 1 2 4 3<br>3 3 3 3 3 3 3 3 3 3 3 3 3 3 3 3 3 3 3 3 | | 10000 | 3600.02 | 2307 | 3600 | 17739 | 206 | 2307 |
| (20, 1, 3)(4) | 6 7 7 4 7 7 5 7 7 7 8 5 4 8 6 8 5 5 6 7<br>3 3 2 2 3 1 3 1 1 1 4 3 2 2 4 2 3 4 4 3<br>3 3 3 3 3 3 3 3 3 3 3 3 3 3 3 3 3 3 3 3 | | 10000 | 3600.02 | 2124 | 3031 | 18309 | 215 | 2154 |
| (20, 1, 3)(5) | 6 7 7 7 4 7 7 5 6 8 4 5 6 6 7 4 4 4 4 6<br>4 3 3 3 4 2 3 1 1 3 3 4 4 1 2 3 3 1 4 3<br>3 3 3 3 3 3 3 3 3 3 3 3 3 3 3 3 3 3 3 3 | | 10000 | 3600.22 | 2133 | 109 | 17853 | 209 | 2204 |
| (20, 1, 3)(6) | 4 7 6 7 6 5 7 4 5 4 5 6 8 7 4 5 5 8 7 7<br>1 2 1 2 2 3 1 2 3 4 3 4 1 3 4 3 2 3 4 3<br>3 3 3 3 3 3 3 3 3 3 3 3 3 3 3 3 3 3 3 3 | | 10000 | 3600.13 | 2174 | 2952 | 17796 | 209 | 2293 |
| (20, 1, 3)(7) | 7 5 4 6 6 4 5 4 8 8 5 7 6 5 6 6 5 4 6 5<br>4 3 2 1 2 2 1 4 3 2 2 1 2 3 1 1 2 3 4 2<br>3 3 3 3 3 3 3 3 3 3 3 3 3 3 3 3 3 3 3 3 | | 10000 | 3600.04 | 2171 | 2379 | 17169 | 200 | 2264 |
| (20, 1, 3)(8) | 5 4 7 6 7 6 4 8 4 8 5 8 4 4 7 7 5 5 5 8<br>1 4 1 3 3 4 1 4 4 4 1 2 3 3 2 2 2 3 3 2<br>3 3 3 3 3 3 3 3 3 3 3 3 3 3 3 3 3 3 3 3 | | 10000 | 3600.04 | 2330 | 3600 | 17853 | 209 | 2216 |
| (20, 1, 3)(9) | 5 8 7 8 8 6 5 4 7 8 4 8 8 7 7 5 6 4 6 5<br>4 4 4 3 3 1 4 1 3 3 4 4 1 3 4 3 1 2 3 4<br>3 3 3 3 3 3 3 3 3 3 3 3 3 3 3 3 3 3 3 3 | | 10000 | 3600.13 | 2161 | 146 | 18765 | 219 | 2265 |
| (20, 2, 1)(1) | 4 8 4 5 6 6 5 6 7 5 4 7 7 7 7 8 4 4 6 5<br>4 1 3 2 4 1 1 1 4 4 3 1 1 4 1 4 2 2 2 2<br>1 1 1 1 1 1 1 1 1 1 1 1 1 1 1 1 1 1 1 1 | 5 4 5 5 4 5 5 4 5 4 4 5 5 4 4 4 4 5 5 5 | 16880 | 3600.11 | 2836 | 243 | 22692 | 263 | 2901 |
| (20, 2, 1)(2) | 8 8 5 8 4 8 6 4 5 7 6 4 6 8 5 5 6 6 8 4<br>4 3 1 1 2 4 2 2 1 4 2 1 1 2 2 3 1 4 4 1<br>1 1 1 1 1 1 1 1 1 1 1 1 1 1 1 1 1 1 1 1 | 4 4 5 5 4 4 4 4 5 4 4 5 5 4 4 4 4 4 5 4 | 16880 | 3600.03 | 2960 | 3600 | 22630 | 263 | 2917 |
| (20, 2, 1)(4) | 6 8 6 5 5 4 4 6 8 6 6 6 4 5 4 6 7 4 5 6<br>1 1 2 2 3 4 2 4 1 2 4 1 1 1 1 3 2 1 2 3<br>1 1 1 1 1 1 1 1 1 1 1 1 1 1 1 1 1 1 1 1 | 5 5 5 5 4 4 4 5 4 4 5 5 5 4 4 5 5 4 4 4 | 16880 | 3600.03 | 2933 | 3600 | 22064 | 256 | 2895 |
| (20, 2, 1)(9) | 5 6 7 6 4 7 4 7 7 4 4 5 7 8 4 4 5 4 6 6<br>1 3 1 1 3 4 2 1 2 4 3 2 1 3 2 1 3 1 4 2<br>1 1 1 1 1 1 1 1 1 1 1 1 1 1 1 1 1 1 1 1 | 4 5 4 5 5 5 5 4 4 4 5 4 5 5 5 5 5 4 5 4 | 16880 | 3600.03 | 2843 | 244 | 22294 | 261 | 3033 |
