# Supplementary material for: An Optimization Case Study for solving a Transport Robot Scheduling Problem on Quantum-Hybrid and Quantum-Inspired Hardware
Source: arXiv:2309.09736 source file (2023-10-24)
Supplement: Supplementary file 2 [file Supplementary-Material.pdf]

# S1 Models

All models shown in this section use the following problem parameters:

- machines: $M_1$ (water mixer), $M_2$ (sample shaker), $M_3$ (photo booth),
- samples: $j \in \{1, 2, 3 \ldots, N\}$,
- machine processing times: $p_{j,m}$ for $j \in \{1, \ldots, N\}$, $m \in \{1, 2, 3\}$,
- time (slots): $t \in \{0, \ldots, T-1\}$,
- photos: $k \in \{1, \ldots, K\}$,
- gap between photos $k$ and $k+1$ of sample $j \in \{1, \ldots, N\}$: $g_{j,k}$ for $k \in \{1, \ldots, K-1\}$.

## S1.1 QUBO Model

### S1.1.1 Variables

The quadratic unconstrained binary optimization (QUBO) model uses the variables

$$x_{j,m,t} := \begin{cases} 1, & \text{if sample } j \text{ starts processing on machine } M_m \text{ at time } t, \\ 0, & \text{otherwise} \end{cases} \tag{S1}$$

with $x_{j,m,t} \in \{0, 1\}$ for all $j \in \{1, \ldots, N\}$, $m \in \{1, 2, 3\}$ and $t \in \{1, \ldots, T-1\}$. Here,

$$T := T(N, K, p, g) := \left( \sum_{j=1}^{N} p_{j,1} + p_{j,2} + K \cdot p_{j,3} \right) + \left( \sum_{j=1}^{N} \sum_{k=1}^{K-1} g_{j,k} \right) + N \cdot (3 + K) \tag{S2}$$

is the time horizon for an instance with parameters $N$, $K$, $p := \{p_{j,m} \mid j \in \{1, \ldots, N\},\ m \in \{1, 2, 3\}\}$, $g := \{g_{j,k} \mid j \in \{1, \ldots, N\}, k \in \{1, \ldots, K-1\}\}$.

In total, there are $N \cdot 3 \cdot T(N, K, p, g)$ binary variables. However, a certain subset of these variables can by definition be fixed to 0 to reduce the number of effective optimization variables:

i) The processing of any job on machines $M_1$, $M_2$ and $M_3$ can only start after the preceding processes are finished. Thus, for all $j \in \{1, \ldots, N\}$ and $m \in \{1, 2, 3\}$ we set

$$x_{j,m,t} = 0 \quad \forall t: \ 0 \leq t \leq m - 1 + \sum_{m'=1}^{m-1} p_{j,m'}. \tag{S3}$$

ii) Analogously the latest start for a process on machines $M_1$ and $M_2$ can be bounded by $T-1$ minus the total time taken by the subsequent processes. For all jobs $j = 1, \ldots, N$ and $m = 1, 2$ we set

$$x_{j,m,t} = 0 \quad \forall t: \ (T-1) - \left( \sum_{k=1}^{K-1} g_{j,k} + K \cdot p_{j,3} + \sum_{m'=m}^{2} (1 + p_{j,m'}) \right) \leq t \leq T - 1. \tag{S4}$$

Summarized, $c(N, K, p, g)$ variables are required to attain a constant value of zero to achieve feasibility with $c(N, K, p, g)$ being the number of variables set to zero according to Eqs. (S3) and (S4). Consequently, we arrive at a QUBO with

$$n := N \cdot 3 \cdot T(N, K, p, g) - c(N, K, p, g) \tag{S5}$$

binary optimization variables $x_{j,m,t}$.

### S1.1.2 Constraints

In the following, we write $x$ for the vector consisting of these $n$ optimization variables in an arbitrary but fixed order.

With this notation, the penalty terms for the QUBO read:

1) Each sample is processed precisely once by $M_1$ and $M_2$.

$$P_1(x) := \sum_{j=1}^{N} \sum_{m=1}^{2} \left[ \left( \sum_{t=1}^{T-1} x_{j,m,t} \right) - 1 \right]^2 . \tag{S6}$$

2) All samples are processed $K$ times by the photo booth $M_3$.

$$P_2(x) := \sum_{j=1}^{N} \left[ \left( \sum_{t=1}^{T-1} x_{j,3,t} \right) - K \right]^2 . \tag{S7}$$

3) No two processings can start at the same time (because processings start immediately when a sample is brought to a machine).

$$P_3(x) := \sum_{t=0}^{T-1} \left( \sum_{j=1}^{N} \sum_{m=1}^{3} x_{j,m,t} \right) \left[ \left( \sum_{j=1}^{N} \sum_{m=1}^{3} x_{j,m,t} \right) - 1 \right] . \tag{S8}$$

4) A machine $M_m$ is occupied in the time frame between $t$ and $t + p_{j,m}$ in the case that any sample $j$ has been put on it at time $t$.

$$P_4(x) := \sum_{m=1}^{3} \sum_{j=1}^{N} \sum_{t=0}^{T-1} \left( x_{j,m,t} \cdot \sum_{j \neq j'=1}^{N} \sum_{t'=t+1}^{\min\{t+p_{j,m}, T-1\}} x_{j',m,t'} \right) \tag{S9}$$

5) Processing of a sample on consecutive machines must not overlap.

$$P_5(x) := \sum_{m=1}^{2} \sum_{j=1}^{N} \sum_{t=0}^{T-1} \left( x_{j,m+1,t} \cdot \sum_{t'=\max\{t-p_{j,m}, 0\}}^{T-1} x_{j,m,t'} \right) \tag{S10}$$

6) After a sample is processed at machine $M_2$, it needs to be immediately brought to the photo booth, and the subsequent photos need to be taken at specific times later.

   Let $\gamma_{j,k} := 1 + \sum_{k'=1}^{k-1} g_{j,k'} + p_{j,3} \cdot (k-1)$ for $k \in \{1, \ldots, K\}$ be the desired gap between the end of the shaking process on $M_2$ and start of the $k$th photo on $M_3$. Set

$$P_6(x) := \sum_{j=1}^{N} \sum_{k=1}^{K} \sum_{t=0}^{T-1-\gamma_{j,K}} x_{j,2,t} \cdot (1 - x_{j,3,t+\gamma_{j,k}+p_{j,2}}) . \tag{S11}$$

7) Certain pairs of tasks require a gap of one time unit between them for the robot to travel between the machines and the rack empty-handed. We set $P_7 := P_{7.1} + P_{7.2} + P_{7.3}$ where $P_{7.1}$, $P_{7.2}$ and $P_{7.3}$ are defined as follows:

   7.1) If a job $j$ is put on a machine $M_m$ at time $t$, then no job can be put on any machine at time $t+1$.

$$P_{7.1}(x) := \sum_{t=0}^{T-2} \left( \sum_{j=1}^{N} \sum_{m=1}^{3} x_{j,m,t} \cdot \sum_{j'=1}^{N} \sum_{m'=1}^{3} x_{j',m',t+1} \right) \tag{S12}$$

   7.2) If a job $j$ is picked up from a machine $M_m$ at time $t$, then no other job $j'$ can be picked up from any other machine at times $t$ and $t+1$.

$$P_{7.2}(x) := \sum_{t=0}^{T-2} \sum_{j=1}^{N} \left( \sum_{m=1}^{3} x_{j,m,t-p_{j,m}} \cdot \sum_{j'=1}^{N} \sum_{\substack{m'=1 \\ m' \neq m}}^{3} (x_{j',m',t-p_{j',m'}} + x_{j',m',t+1-p_{j',m'}}) \right) \tag{S13}$$

7.3) If a job $j$ is picked up from a machine $M_m$ at time $t$, then no other job can be put on any machine at times $t$ and $t+1$.

$$P_{7.3}(x) := \sum_{t=0}^{T-1} \sum_{m=1}^{3} \left( \sum_{j=1}^{N} x_{j,m,t-p_{j,m}} \cdot \sum_{\substack{j'=1 \\ j' \neq j}}^{N} \sum_{m'=1}^{3} (x_{j',m',t} + x_{j',m',t+1}) \right) \tag{S14}$$

#### S1.1.3 Objective

The objective function computes as

$$F(x) := \sum_{j=1}^{N} \sum_{t=1}^{T-1} \left( t + p_{j,2} + 1 + K \cdot p_{j,3} + \sum_{k=1}^{K-1} g_{j,k} + 1 \right) \cdot x_{j,2,t} \,. \tag{S15}$$

#### S1.1.4 Summary

Altogether, the *QUBO model* is defined as:

$$\begin{aligned} \min_{x} \quad & \rho_0 F(x) + \sum_{i=1}^{7} \rho_i P_i(x) \\ \text{s.t.} \quad & x \in \{0,1\}^n \end{aligned} \tag{S16}$$

### S1.2 Sequence Model

#### S1.2.1 Variables

We define the event set $E := \{(j,i,a) \mid j \in \{1,\ldots,N\},\ i \in \{1,\ldots,2+K\},\ a \in \{0 \text{ (place)}, 1 \text{ (pick up)}\}\}$, where event

$$(j,i,a) \text{ represents action } a \text{ for sample } j \begin{cases} \text{on machine } i & \text{for } i \leq 2; \\ \text{at the camera for photo } i-2 & \text{for } i \geq 3. \end{cases} \tag{S17}$$

The following variables are used in the sequence model:

- $\tau_e \in \mathbb{R}_{\geq 0}$: Time of event $e$ for all $e \in E$.
- $\delta_{m,j,j'} = \begin{cases} 1, & \text{if sample } j \text{ is processed by machine } m \text{ before sample } j' \,, \\ 0, & \text{otherwise} \,, \end{cases}$
  for all $m \in \{1,2\}$, $j,j' \in \{1,\ldots,N\}$, $j \neq j'$.
- $\varepsilon_{e,f} = \begin{cases} 1, & \text{if event } e \text{ happens before event } f \,, \\ 0, & \text{otherwise} \,, \end{cases}$
  for all $e = (j,i,a), f = (j',i',a') \in E$, $j \neq j'$, $i \neq i'$, $\min\{i,i'\} \leq 2$.
- $\zeta_{k,j,k',j'} = \begin{cases} 1, & \text{if the } k\text{th photo of sample } j \text{ is taken before the } k'\text{th photo of sample } j' \,, \\ 0, & \text{otherwise} \,, \end{cases}$
  for all $j,j' \in \{1,\ldots,N\}$, for all $k,k' \in \{1,\ldots,K\}$ with $j \neq j'$, $k \neq k'$.

#### S1.2.2 Constraints

To formulate the constraints we introduce the following notation:

- For $j \in \{1,\ldots,n\}$ and $k \in \{1,\ldots,K\}$ we denote by $\gamma_{j,k} := 1 + \sum_{k'=1}^{k-1} g_{j,k'} + (k-1) \cdot p_{j,3}$ the gap between the end of the shaking process of sample $j$ and the beginning of the process of the $k$th photo.
- $\Gamma := \sum_{j=1}^{N} \left[ \left( \sum_{m=1}^{3} p_{j,i} + 1 \right) + \gamma_{j,K} + 1 \right]$ is a sufficiently large constant that is used for the "Big M" method (Griva, Nash, Sofer 2009).

Then we define the following list of constraints:

1) No two samples are processed on neither the water mixer nor the sample shaker at the same time.

$$\delta_{m,j,j'} + \delta_{m,j',j} = 1 \qquad \forall m \in \{1,2\},\ j,j' \in \{1,\dots,N\},\ j \neq j'. \tag{$C_1$}$$

2) The robot cannot perform two events of different samples at different places at the same time.

$$\varepsilon_{e,f} + \varepsilon_{f,e} = 1 \qquad \forall e = (j,i,a), f = (j',i',a') \in E,\ j \neq j',\ i \neq i'. \tag{$C_2$}$$

3) No two samples can be at the photo booth for different photos at the same time.

$$\zeta_{k,j,k',j'} + \zeta_{k',j',k,j} = 1 \qquad \forall j,j' \in \{1,\dots,N\},\ k,k' \in \{1,\dots,K\},\ j \neq j',\ k \neq k'. \tag{$C_3$}$$

4) The sample must be picked up exactly after its processing time.

$$\tau_{(j,i,1)} = \tau_{(j,i,0)} + p_{j,i} \qquad \forall j \in \{1,\dots,N\},\ i \in \{1,2\}. \tag{$C_4$}$$

5) The transportation time of 1 time unit must be waited for.

$$\tau_{(j,i',0)} \geq \tau_{(j,i,1)} + 1 \qquad \forall j \in \{1,\dots,N\},\ i,i' \in \{1,\dots,2+K\},\ i' > i. \tag{$C_5$}$$

6) The time frames at water mixer and sample shaker must match the orders specified by the $\delta$-variables. The robot must first bring a sample away and can then get another one.

$$\tau_{(j',i,0)} \geq \tau_{(j,i,1)} + 2 - \Gamma \cdot \delta_{i,j',j} \qquad \forall i \in \{1,2\},\ j,j' \in \{1,\dots,N\},\ j \neq j'. \tag{$C_6$}$$

7) The $k$th photos of different samples must not overlap.

$$\tau_{(j',2+k,0)} \geq \tau_{(j,2+k,1)} + 2 - \Gamma \cdot \delta_{2,j',j} \qquad \forall j,j' \in \{1,\dots,N\},\ j \neq j',\ k \in \{1,\dots,K\}. \tag{$C_7$}$$

8) Different photos of different samples must not overlap.

$$\tau_{(j',2+k',0)} \geq \tau_{(j,2+k,1)} + 2 - \Gamma \cdot \zeta_{k',j',k,j} \qquad \forall j,j' \in \{1,\dots,N\},\ k,k' \in \{1,\dots,K\},\ j \neq j',\ k \neq k'. \tag{$C_8$}$$

9) The times of the events of different samples at different machines must match the order and the robot must have enough time in between.

$$\tau_f \geq \tau_e - \Gamma \cdot \varepsilon_{f,e} + 2 \qquad \forall e = (j,i,1), f = (j',i',a') \in E,\ j \neq j',\ i \neq i',\ \min\{i,i'\} \leq 2. \tag{$C_{9.1}$}$$

$$\tau_f \geq \tau_e - \Gamma \cdot \varepsilon_{f,e} + 2 \qquad \forall e = (j,i,a), f = (j',i',0) \in E,\ j \neq j',\ i \neq i',\ \min\{i,i'\} \leq 2. \tag{$C_{9.2}$}$$

$$\tau_f \geq \tau_e - \Gamma \cdot \varepsilon_{f,e} + 1 \qquad \forall e = (j,i,0), f = (j',i',1) \in E,\ j \neq j',\ i \neq i',\ \min\{i,i'\} \leq 2. \tag{$C_{9.3}$}$$

10) The photo times must have the correct distance to the end of the shaking process.

$$\tau_{(j,2+k,0)} = \tau_{(j,2,1)} + \gamma_{j,k} \qquad \forall j \in \{1,\dots,N\},\ k \in \{1,\dots,K\}. \tag{$C_{10.1}$}$$

$$\tau_{(j,2+k,1)} = \tau_{(j,2,1)} + \gamma_{j,k} + p_{j,3} \qquad \forall j \in \{1,\dots,N\},\ k \in \{1,\dots,K\}. \tag{$C_{10.2}$}$$

### S1.2.3 Objective

The objective function computes as

$$F(\tau,\delta,\varepsilon,\zeta) := \sum_{j=1}^{N} (\tau_{(j,2+K,1)} + 2). \tag{S18}$$

Note that by definition of the model, it is a valid solution that a sample is placed at time 0 on machine $M_1$, which implies that the robot transports the sample at time $-1$ from the rack to $M_1$. To overcome this we add an extra $+1$ to each sample to shift the whole schedule to the right. This does not affect the optimization process itself, but is rather a linear translation of the whole schedule w.r.t. the objective function to get a schedule starting at 0 in compliance with the other models. Lastly the sample arrives at the rack one time unit after the $K$'th photo has been shot, thus we add another $+1$.

### S1.2.4 Summary

Altogether, the *sequence model* is defined as:

$$\begin{aligned}
\min_{\tau,\delta,\varepsilon,\zeta} \quad & F(\tau,\delta,\varepsilon,\zeta) \\
\text{s.t.} \quad & C_1,\dots,C_8, C_{9.1}, C_{9.2}, C_{9.3}, C_{10.1}, C_{10,2} \\
& \tau_e \in \mathbb{R}_{\geq 0}\ \forall e \in E \\
& \delta_{m,j,j'} \in \{0,1\}\ \forall m \in \{1,2\}, j,j' \in \{1,\dots,N\},\ j \neq j' \\
& \varepsilon_{e,f} \in \{0,1\}\ \forall e=(j,i,a), f=(j',i',a') \in E,\ j\neq j',\ i \neq i', \min\{i,i'\} \leq 2 \\
& \zeta_{k,j,k',j'} \in \{0,1\}\ \forall j,j' \in \{1,\dots,N\},\ \forall k,k' \in \{1,\dots,K\} \text{ with } j \neq j', k \neq k'
\end{aligned} \tag{S19}$$

## S1.3 Time-Indexed Model

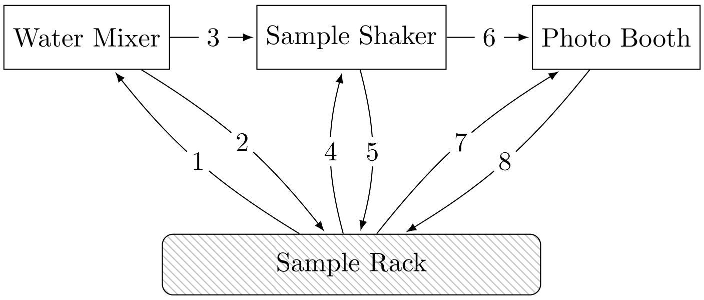


**Supplementary Figure S1.** Numbering of the eight different routes the transport robot can move along between the machines and the rack.

### S1.3.1 Variables

The time-indexed model makes use of the binary variables

$$y_{j,r,t} := \begin{cases} 1, & \text{if sample } j \text{ is transported by the robot on route } r \text{ at time } t\ , \\ 0, & \text{otherwise} \end{cases} \tag{S20}$$

for all $j \in \{1,\dots,N\}$, $r \in \{1,\dots,8\}$ and $t \in \{0,\dots,T-1\}$, where the routes $r$ are given by Fig. S1. The time horizon $T$ is defined as in Eq. (S2). Additionally we have variables $z_j \in \mathbb{R}_{\geq 0}$ for $j \in \{1,\dots,N\}$ that are used to define the objective function (see Eq. (S21)).

Setting $M_0$ to be the rack we define $r^-(i)$ to be the set of incoming routes and $r^+(i)$ the set of outgoing routes of $M_i$ for $i \in \{0,1,2,3\}$, i.e. $r^-(0) = \{2,5,8\}$, $r^+(0) = \{1,4,7\}$, $r^-(1) = \{1\}$ and so on. The set of all routes is $R := \{1,\dots,8\}$.

### S1.3.2 Constraints

We define the following constraints:

1) The transport robot can carry at most one sample at a time.

$$\sum_{j=1}^{N}\sum_{r=1}^{8} y_{j,r,t} \leq 1 \qquad \forall t \in \{0,\dots,T-1\}. \tag{$C_1$}$$

2) The transport robot cannot teleport from one machine to another. For every time $t$ and every machine $i$ the robot cannot serve some route to $i$ during $(t,t+1)$ and a route starting from another machine during $(t+1,t+2)$.

$$\sum_{j=1}^{N}\left[\left(\sum_{r\in r^-(i)} y_{j,r,t}\right) + \sum_{r \in R\setminus r^+(i)} y_{j,r,t+1}\right] \leq 1 \qquad \forall i \in \{0,\dots,3\},\ t \in \{0,\dots,T-2\}. \tag{$C_2$}$$

3) Every machine may be occupied by at most one sample.

$$\sum_{j=1}^{N}\sum_{t'=0}^{t}\left[\left(\sum_{r\in r^-(i)} y_{j,r,t'}\right) - \sum_{r\in r^+(i)} y_{j,r,t'}\right] \leq 1 \qquad \forall i \in \{1,2,3\},\ t \in \{0,\dots,T-1\}. \tag{$C_3$}$$

4) Every sample is transported to the water mixer $M_1$ exactly once.

$$\sum_{t=0}^{T-1} y_{j,1,t} = 1 \qquad \forall j \in \{1,\dots,N\}. \tag{$C_4$}$$

5) Samples can only be picked up from a machine, when they have been brought to it and stayed there for the appropriate time.

$$\sum_{t'=0}^{t}\sum_{r\in r^+(i)} y_{j,r,t'} = \sum_{t'=0}^{t-p_{i,j}-1}\sum_{r\in r^-(i)} y_{j,r,t'} \qquad \forall j \in \{1,\dots,N\},\ i \in \{1,2,3\},\ t \in \{0,\dots,T-1\}. \tag{$C_5$}$$

6) Routes between rack and the first two machines must be driven along in the correct order.

$$\sum_{t'=0}^{t} y_{j,4,t'} \leq \sum_{t'=0}^{t-1} y_{j,2,t'} \qquad \forall j \in \{1,\dots,N\},\ t \in \{0,\dots,T-1\}. \tag{$C_6$}$$

7) At no time has a sample been brought from the rack to the camera more often than from the camera or the shaker to the rack.

$$\sum_{t'=0}^{t} y_{j,7,t'} \leq \sum_{t'=0}^{t-1}(y_{j,5,t'} + y_{j,8,t'}) \qquad \forall j \in \{1,\dots,N\},\ t \in \{0,\dots,T-1\}. \tag{$C_7$}$$

8) A sample is picked up from the camera at time $t$ if and only if it has been placed there at time $t-p_{j,3}$, i. e., $y_{j,8,t} = 0$ for $t \leq p_{j,3}$ and $y_{j,8,t} = y_{j,6,t-p_{j,3}-1} + y_{j,7,t-p_{j,3}-1}$ for $t > p_{j,3}$. These constraints are equivalent to

$$\sum_{t'=0}^{t} y_{j,8,t'} = \sum_{t'=0}^{t-p_{j,3}-1} (y_{j,6,t'} + x_{j,7,t'}) \qquad \forall j \in \{1,\dots,N\},\ t \in \{0,\dots,T-1\}. \tag{$C_8$}$$

9) Every sample has to be picked up from the shaker early enough for the last photo.

$$\sum_{t=0}^{T-1-p_{j,3}-\gamma_{j,K}} (y_{j,5,t} + y_{j,6,t}) = 1 \qquad \forall j \in \{1,\dots,N\}. \tag{$C_9$}$$

10) Every sample has to be picked up from the camera the same number of times as it is placed there.

$$\sum_{t=0}^{T-1}(y_{j,6,t} + y_{j,7,t} - y_{j,8,t}) = 0 \qquad \forall j \in \{1,\dots,N\}. \tag{$C_{10}$}$$

11) Samples must be at the camera at photo dates.

$$y_{j,5,t} + y_{j,6,t} \leq \sum_{t'=0}^{t+\gamma_{j,k}-1} (y_{j,6,t'} + y_{j,7,t'}) - \sum_{t'=0}^{t+\gamma_{j,k}+p_{j,3}-1} y_{j,8,t'} \qquad \forall j \in \{1,\dots,N\},$$
$$k \in \{1,\dots,K\},\ t \in \{0,\dots,T-\gamma_{j,k}-p_{j,3}\}. \tag{$C_{11}$}$$

12) Lastly we define a constraint that bounds the objective variables $z_j$ below by the arrival time of sample $j$ at the rack after the schedule has finished.

$$(t+1)\cdot y_{j,8,t} \leq z_j \qquad \forall j \in \{1,\dots,N\},\ t \in \{0,\dots,T-1\}, \tag{$C_F$}$$

### S1.3.3 Objective

Let $y, z$ be vectors achieved by writing the corresponding variables into a vector in some arbitrary but fixed order. Using the constraint $C_F$, Eq. ($C_F$), the objective function simply computes as

$$F(y,z) := \sum_{j=1}^{N} z_j . \tag{S21}$$

### S1.3.4 Summary

Altogether, the *time-indexed model* is defined as:

$$\begin{aligned} \min_{y,z} \quad & F(y,z) \\ \text{s.t.} \quad & C_1, \ldots, C_{11}, C_F \\ & y_{j,r,t} \in \{0,1\} \; \forall j \in \{1,\ldots,N\}, r \in \{1,\ldots,8\}, t \in \{0,\ldots,T-1\} \\ & z_j \in \mathbb{R}_{\geq 0} \; \forall j \in \{1,\ldots,N\} \end{aligned} \tag{S22}$$

# S2 Benchmark Library

It is our goal to define a representative benchmark library with meaningful instances. For this purpose, we specify a set of relevant values for each parameter as listed in Table S1. We consider all 120 parameter combinations $N \in D_N$, $K \in D_K$ and $p_3 \in D_{p_3}$. For each combination, the remaining parameters are then drawn uniformly from the corresponding set of allowed values 10 times, which leads to 1200 instances in total.

**Supplementary Table S1.** Parameter configurations for our benchmark instances.

| Parameter | Choice | Domain |
|---|---|---|
| $N$ | all | $D_N := \{1, 2, \ldots, 10, 15, 20, 25, 50, 100\}$ |
| $K$ | all | $D_K := \{1, 2, 3, 4\}$ |
| $p_3$ | all | $D_{p_3} := \{1, 3\}$ |
| $p_{j,1}$ | random | $D_{p_1} := \{4, 5, 6, 7, 8\}$ |
| $p_{j,2}$ | random | $D_{p_2} := \{1, 2, 3, 4\}$ |
| $g_{j,1}$ | random | $D_{g_1} := \{4, 5\}$ |
| $g_{j,2}$ | random | $D_{g_2} := \{8, \ldots, 12\}$ |
| $g_{j,3}$ | random | $D_{g_3} := \{16, \ldots, 24\}$ |

However, we filter these instances such that only a relevant subset remains. Specifically, we only keep the instances with at least 2071 and at most 22 692 binary variables in the corresponding QUBO formulation from Section 2.2.2. This excludes the very easy and the very hard cases. A complete list with all computed instances, their parameters and the benchmark results is appended as supplementary material as well.

We collect groups of instances $(N, K)$ that have the same number of samples $N$ and photos $K$. In Table S2, we list how many instances each group contains. Additionally in Fig. S2 the number of variables per instance in the QUBO formulation and group is shown in a scatter plot fashion.

# S3 Fujitsu Solver Settings

Both Fujitsu's digital annealer (FDA) and Fujitsu's digital annealer hybrid framework (FDAh) have various parameters that can be used to tune the solver runs. Table S3 and Table S4 contain the values for each parameter of both solvers that was used in the benchmark.

# S4 Pre-study

Before we started with the actual benchmarks for this paper, we performed a small pre-study in which we exemplarily tested our solver candidates on a few instances to assess their overall behavior. This allowed us

**Supplementary Table S2.** Size informations about the instance groups: Number of instances as well as minimum and maximum number of variables for the the corresponding QUBO formulation.

| $(N, K)$ | Num. instances | Min num. vars | Max num. vars |
|---|---|---|---|
| $(4, 4)$ | 19 | 2096 | 2488 |
| $(5, 3)$ | 15 | 2071 | 2494 |
| $(5, 4)$ | 20 | 3384 | 4118 |
| $(6, 3)$ | 20 | 2849 | 3834 |
| $(6, 4)$ | 20 | 4935 | 6109 |
| $(7, 3)$ | 20 | 4022 | 5146 |
| $(7, 4)$ | 16 | 6787 | 8080 |
| $(8, 3)$ | 20 | 5215 | 6880 |
| $(9, 3)$ | 11 | 6750 | 8042 |
| $(8, 4)$ | 4 | 10 822 | 11 058 |
| $(9, 4)$ | 20 | 11 590 | 14 106 |
| $(10, 3)$ | 1 | 11 026 | 11 026 |
| $(10, 4)$ | 20 | 14 307 | 17 580 |
| $(15, 2)$ | 20 | 12 270 | 16 129 |
| $(15, 3)$ | 10 | 19 775 | 20 581 |
| $(20, 1)$ | 20 | 14 541 | 18 765 |
| $(20, 2)$ | 4 | 22 064 | 22 692 |

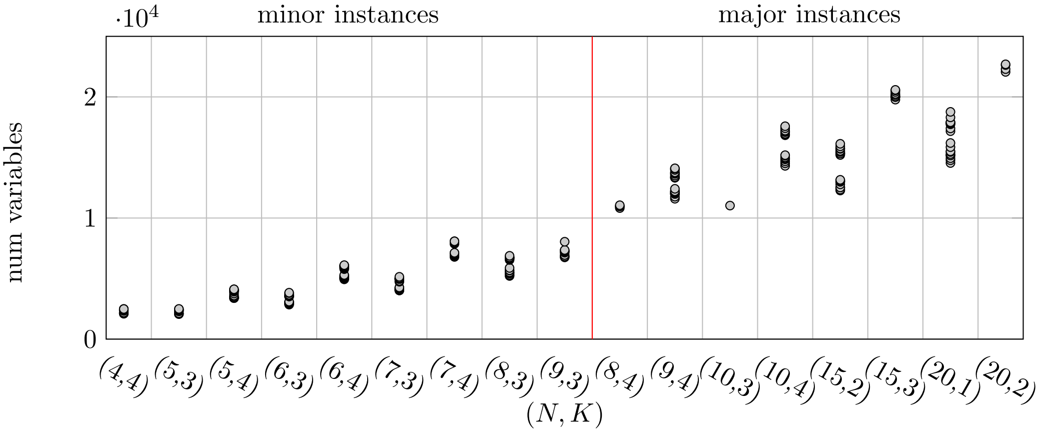


**Supplementary Figure S2.** The number of variables of each group $(N, K)$ of instances. The minor instances are left to the red vertical line, the major instances to the right.

to exclude three potential solver candidates beforehand. In this appendix section, we briefly summarize our qualitative observations for these excluded solvers:

- First, it turned out that quantum approximate optimization algorithm (QAOA) on the IBM gate-based quantum computers (IBM Quantum 2023) is very limited in problem size (up to $\sim 10^2$ variables) and, in addition, has an end-to-end runtime that is magnitudes longer than that of all other solvers due to the queuing system of the cloud service which can lead to major delays.
- Second, Quera's Rydberg quantum computer *Aquila* (Wurtz *et al.* 2023) does not support local detuning, which is necessary for the QUBO encoding from (Nguyen *et al.* 2023), and we did not find an alternative mixed integer program (MIP) representation of our use case.
- Third, Toshiba's Simulated Bifurcation Machine (TSB) had a very bad performance on all test instances and did not yield feasible solutions.

**Supplementary Table S3.** FDA parameters. Here, $k_{\text{iter}}$ denotes the number of iterations for FDA with the QUBO model (QU-FDA) as declared in the column "Minor instance limit" of Table 1.

| Parameter | Value |
|---|---|
| "access_profile_file" | "AUTO" |
| "processor" | "DAv2" |
| "connection_mode" | "async" |
| "DAv2_optimization_method" | "annealing" |
| "DAv2_number_iterations" | $k_{\text{iter}}$ |
| "DAv2_number_runs" | 32 |
| "DAv2_temperature_start" | 10 000 |
| "DAv2_temperature_end" | 10 |
| "DAv2_temperature_mode" | 0 |
| "DAv2_temperature_interval" | $k_{\text{iter}}/1\,000\,000$ |
| "DAv2_offset_increase_rate" | 100 |
| "DAv2_solution_mode" | "COMPLETE" |
| "DAv2_bit_precision" | 16 |

**Supplementary Table S4.** FDAh parameters. Here, $k_{\text{time}}$ denotes the time limit for FDAh with the QUBO model (QU-FDAh) as declared in the column "Major instance limit" of Table 1.

| Parameter | Value |
|---|---|
| "access_profile_file" | "AUTO" |
| "processor" | "DAv3" |
| "connection_mode" | "async" |
| "DAv3_time_limit_sec" | $k_{\text{time}}$ |
| "DAv3__use__target_energy" | "False" |
| "DAv3_target_energy" | 0 |
| "DAv3_num_solution" | 16 |
| "DAv3_num_group" | 4 |
| "DAv3_num_output_solution" | 5 |
| "DAv3_gs_num_iteration_factor" | 5 |
| "DAv3_gs_num_iteration_cl" | 200 |
| "DAv3_gs_penalty_auto_mode" | 1 |
| "DAv3_gs_penalty_coef" | 1 |
| "DAv3_gs_penalty_inc_rate" | 150 |
| "DAv3_gs_max_penalty_coef" | 0 |

# References

Griva, I., Nash, S., Sofer, A., 2009. *Linear and Nonlinear Optimization: Second Edition*. Other Titles in Applied Mathematics. Society for Industrial, Applied Mathematics (SIAM, 3600 Market Street, Floor 6, Philadelphia, PA 19104).

IBM Quantum, 2023. Ibm quantum services. https://quantum-computing.ibm.com. Last accessed 2023-01-31.

Nguyen, M.-T. *et al.*, 2023. Quantum optimization with arbitrary connectivity using rydberg atom arrays. *PRX Quantum*. 4.1, 010316. https://doi.org/10.1103/PRXQuantum.4.010316.

Wurtz, J. *et al.*, 2023. Aquila: quera's 256-qubit neutral-atom quantum computer. arXiv preprint 2306.11727. https://doi.org/10.48550/arXiv.2306.11727.
